# Supplementary material for: On the Optimization and Generalization of Two-layer Transformers with Sign Gradient Descent
Source: arXiv:2410.04870 source file (2025-03-02)
Supplement: Supplementary file 1 [file comparison.tex]

\newpage
\section{Comparison with the related works}

% \paragraph{Comparison with~\cite{JSL22}}

% This work parametrize the pre-softmax attention weights matrix and simplify this $L \times L$ matrix to 3 quantities: the elements at diagonal (fixed), in the same group, and in different groups, sine they claim the gradients of elements in the same category are identical (with population loss as optimization objective).
% The reason they claim is that the data is symmetric. More formally, patches in one data point have same distribution, which implies data distribution keep unchanged under permutation across patches. Note the difference between the permutation invariance in~\citep{JSL22} and Remark~\ref{remark:permutation-to-parameter-grad}. 
% The former is talking about different patch pair has same gradients, i.e., $\frac{\partial F}{\partial z_{i,j}} = \frac{\partial F}{\partial z_{k,l}}$ 
% % (we particularity care about $(k,l) = (j,i)$)
% , while the latter is talking about the gradient is invariant under permutation, i.e., $\frac{\partial F}{\partial z_{i,j}} = \frac{\partial \Tilde{F}}{\partial z_{\pi(i),\pi(j)}}$.
% In our setting, there is no difference if we use symmetric data because we take average across all token positions and channel dimensions after attention operation. 

\paragraph{Comparison with Li et al.~\cite{LWLC23}}

Li et al.~\cite{LWLC23} uses $\Wv_Q,\Wv_K,\Wv_V$ parameterization in their analysis which is close to practice. 
They divides tokens in one sample into three groups: the label-relevant tokens, confusion tokens, and non-discriminative tokens. They bound the query/key vectors and attention weights based on token group.
However, they assume that $\Wv_Q\xv^{(l)}$ is already close to some orthogonal basis, which means that the attention weights are not uniform. 
More specifically, firstly, if $\xv^{(s)}$ and $\xv^{(l)}$ belong to the same group, then the pre-softmax logits $\xv^{(s)\top}\Wv_K^\top\Wv_Q^\top\xv^{(l)}$ would be significantly larger than $\xv^{(s^\prime)\top}\Wv_K^\top\Wv_Q^\top\xv^{(l)}$ at initialization where $\xv^{(s^\prime)}$ and $\xv^{(l)}$ are not in the same group. 
However, randomly initialized $\Wv_Q,\Wv_K$ leads to uniform attention.
Secondly, with the prescribed orthogonal basis, they can decompose query \& key vectors based on this basis and trace the coefficients. 
% In our setting, we can use initialization vectors instead.

% \paragraph{Comparison with~\cite{TWCD23}}

% This paper uses a two-stage analysis. 
% At the first stage, they freeze the attention weights and train the value parameters only. At the second stage, in my understanding, they freeze value parameters at a large timestep $t$ and train attention weights. 
% They also use heavy reparameterization to make the dynamics have some nice properties.
