# Supplementary material for: On the Optimization and Generalization of Two-layer Transformers with Sign Gradient Descent
Source: arXiv:2410.04870 source file (2025-03-02)
Supplement: Supplementary file 2 [file gd.tex]

\section{GD Signal Learning}
\subsection{First Stage}

In the first stage, we want to show attention weights are stuck in initialization while value parameters learns faster.

\begin{lemma}
    Consider the TF model defined in~\ref{def:softmaxattn-linearact-L2-model}. 
    % Let $\wv^{(t)}_{q,s}$ and $\wv^{(t)}_{k,s}$ for $s\in[d_k]$ be the query and key parameters of the TF at the $t$-th iteration of gradient descent. 
    At initialization, we want to show $z_{0,0}, z_{0,1}$, $z_{1,0}, z_{1,1}$ are small.
    Recall that $z_{j,l} = \sum_{r\in[d_k]} \langle\wv_{q,r}, \xv^{(j)}\rangle\langle\wv_{k,r}, \xv^{(l)}\rangle$. 
    Then, with probability at least $1 - \delta$, we have
    \begin{align*}
        \abs{z_{0, 0}} & \leq \sqrt{d_k} \sqrt{2\log(Cd_k/\delta)} \sigma_q\norm{\muv} \cdot \sqrt{2\log(Cd_k/\delta)} \sigma_q\norm{\muv} \\
        \abs{z_{0, 1}} & \leq \sqrt{d_k} \sqrt{2\log(Cd_k/\delta)} \sigma_q\norm{\muv} \cdot 2\sqrt{\log(Cd_kn / \delta)}\sigma_k\sigma_p\sqrt{d} \\
        \abs{z_{1, 0}} & \leq \sqrt{d_k} \sqrt{2\log(Cd_k/\delta)} \sigma_q\norm{\muv} \cdot 2\sqrt{\log(Cd_kn / \delta)}\sigma_k\sigma_p\sqrt{d} \\
        \abs{z_{1, 1}} & \leq \sqrt{d_k} 2\sqrt{\log(Cd_kn / \delta)}\sigma_k\sigma_p\sqrt{d} \cdot 2\sqrt{\log(Cd_kn / \delta)}\sigma_k\sigma_p\sqrt{d}
    \end{align*}
    By \textcolor{red}{some condition}, we have $z_{j,l} = o(1)$ and thus $s_{j,l} = 1/2 + o(1)$ for all $j,l \in \set{0,1}$ and $i\in [n]$.
\end{lemma}
\begin{remark}
    Skip the proof. Roughly speaking, for all except $z_{1,1}$ we use sub-gaussian bound for $\langle \wv, \muv\rangle$ and sub-exponential bound for $\langle \wv, \xiv_i\rangle$. The $\sqrt{d_k}$ is due to independence, but the proof is unclear. The proof for $z_{1,1}$ is also unclear.
\end{remark}

\begin{lemma}[Lemma D.1 in \citep{ccbg22}]
    Assume $s_{ab}^{0} = 1/2$ for $a,b\in[2]$ and $\Wv_{Q, s}, \Wv_{K, s}$ are fixed for all $s \in [m_k]$. If we choose
    \begin{align}
        n \cdot \text{SNR}^q \geq 
        C\log\left(6/\sigma_{0}\norm{\mu}_{2}\right)2^{2q+6}
        [4\log(8mn/\delta)]^{(q-1)/2},
    \end{align}
    where $C = O(1)$ is a positive constant, there exists time 
    \begin{align*}
        T_{1} = \frac{C\log\left(6/\sigma_{0}\norm{\mu}_{2}\right)2^{q+1}m}{\eta\sigma_{0}^{q-2}\norm{\mu}_{2}^{q}}
    \end{align*}
    such that
    \begin{itemize}
        \item $\max_r \gamma_{j,r}^{(T_1)} \geq 2$ for $j \in \set{\pm1}$
        \item $\abs{\rho_{j,r,i}^{(t)}} \leq \sigma_{0}\sigma_{p}\sqrt{d}/2$ for $j \in \set{\pm1},~r\in[m],~i\in[n]$ and $0 \leq t \leq T_{1}$.
    \end{itemize}
\end{lemma}
\begin{remark}
    If attention weights are initialized as $1/2$ and fixed, the proof is the same as in~\citep{ccbg22}. As in~\citep{ccbg22}, the $q$-power nonlinearity on value is necessary to make $\gamma$ and $\rho$ have different speed and separable.
\end{remark}
