# Supplementary material for: On the Optimization and Generalization of Two-layer Transformers with Sign Gradient Descent
Source: arXiv:2410.04870 source file (2025-03-02)
Supplement: Supplementary file 3 [file limitations.tex]

\newpage
\section{Limitations and Broader Impacts}
\label{sec:limitations_etc}

\paragraph{Limitations}
The theoretical results in our works rely on specific data settings and model settings in Section.~\ref{sec:main_preliminaries} and Condition.~\ref{cond:main_condition}.
For the data, we make assumptions about sparsity, orthogonality, and context length. 
Currently, our analysis can only be extended to feature vectors with constant non-zero entries and noise vectors with some non-zero entries.
Although we provide empirical evidences that our theoretical results hold with more relaxed assumptions, we do not provide theory in those cases.
The use of linearly separable data is also a limitation, which makes a linear classifier able to achieve perfect classification.

For the model, we consider a two-layer transformer consisting of one softmax self-attention layer and one fixed linear layer.
It is important to generalize our analysis to multi-head attention,
a full transformer block consisting of one softmax self-attention layer and one fully connected layer,
and even deep transformers.

Although we demonstrate the fast convergence rate of sign gradient descent in our binary classification task and two-layer transformers, this rate may be task- and/or model-specific.
In our setting, sign gradient descent is better on the optimization, but the generalization error of sign gradient descent is large, while that of gradient descent is small. 
It is interesting to generalize our analysis to a case where sign gradient descent is better than gradient descent in terms of both optimization and generalization.
Moreover, the model and task in our work are motivated by vision transformers and image classification. It is important to study the role of sign gradient descent or Adam on casual attention model with language modelling objective.

For the optimizer, we analyze the sign gradient descent in the deterministic setting which is similar to Adam, but it is also important to establish a theory or generalize our analysis to real Adam.

\paragraph{Broader Impacts}
Our work establish an end-to-end theory of learning two-layers transformers with sign gradient descent, taking a step forward towards understanding why Adam is so successful in transformer optimization. 
We hope that our work can
facilitate the improvements on sign-based methods and Adam, and the development of potentially new efficient optimization methods for transformers.
 % We hope that our work will serve as the stepping stone for building a more precise theory of Transformer optimization, as well as contributing to the development of efficient training methods for Transformers.
% or development of optimization methods for Transformers. However, these directions are out-of-scope of this work, and left for future work.
