# Supplementary material for: On the Optimization and Generalization of Two-layer Transformers with Sign Gradient Descent
Source: arXiv:2410.04870 source file (2025-03-02)
Supplement: Supplementary file 4 [file notation.tex]

\section{Notation}
\label{sec:notation}

\paragraph{Data} We consider two patch data $\Xv = \left(\xv^{(1)}, \xv^{(2)}\right) \in \Rb^{d\times2}$, where $\xv^{(1)} = y\muv$ is the feature and $\xv^{(2)} = \xiv$, where $\xiv \sim \mathcal{N}\left(0, \sigma_p^2 \cdot \left(\Iv - \muv\muv^\top \cdot \norm{\muv}^{-2}_2\right)\right)$. The position or permutation will be discussed later after introducing the model. Define $\text{SNR} := \norm{\muv}_{2} / \sigma_p\sqrt{d}$. Suppose we have a training dataset of size $n$, denoted by $\mathcal{S} = \set{(\Xv_i, y_i)}_{i=1}^n$.

\paragraph{Model}
We consider the general case where sequence length is $L$, 
thus $\Xv = \left(\xv^{(1)}, \dots, \xv^{(L)} \right) \in \Rb^{d \times L}$. 
The parameters are $\Wv = \left(\Wv_{Q}, \Wv_{K}, \Wv_{V,j} \right)$, where $\Wv_{Q}, \Wv_{K} \in \Rb^{m_k \times d}$ and $\Wv_{V,j} \in \Rb^{m_v \times d}$ for $j \in \set{\pm 1}$. Define $\wv_{V, j, r} = \Wv_{V,j, (\cdot, r)}^{\top} \in \Rb^{d}$.
Then we define $\mathsf{AttnBinaryV}$ model as:
\begin{align*}
    F_j(\Wv, \Xv) 
    = \frac{1}{m_v}\sum_{l \in [L], r \in [m_v]} \sum_{a=1}^L s_{la} \sigma\left(\left\langle\wv_{V,j,r}, \xv^{(a)}\right\rangle\right),
\end{align*}
where $s_{la} = \softmax{z_{l,1}, \dots z_{l,L}}_{a}$, and 
\begin{align*}
    z_{l, a} 
    = \sum_{s \in [m_k]} \left\langle\wv_{Q,s}, \xv^{(l)}\right\rangle \left\langle\wv_{K,s}, \xv^{(a)}\right\rangle.
\end{align*}
We can also write the model in vector form
\begin{align*}
    F_j(\Wv, \Xv) 
    = \frac{1}{m_v}\sum_{l\in[L]}\textbf{1}^\top \sigma\left(\Wv_{V, j}\Xv\right)\softmax{\Xv^{\top}\Wv_{K}^{\top}\Wv_{Q}\xv^{(l)}} .
\end{align*}
Particularly, when we use $L = 2$ and linear activation, i.e., $\sigma(x) = x$, we have
\begin{align}
    \label{def:softmaxattn-linearact-L2-model}
    F_j(\Wv, \Xv) 
    = \frac{1}{m_v}\sum_{r \in [m_v]} 
    \left[ \left(s_{11} + s_{21}\right)
    \left\langle\wv_{V,j,r}, \xv^{(1)}\right\rangle
    + \left(s_{12} + s_{22}\right) 
    \left\langle\wv_{V,j,r}, \xv^{(2)}\right\rangle
    \right].
\end{align}
Define $\bar{\wv}_{V,j} = \sum_{r\in[m_v]} \wv_{V,j,r} / m_v$. Let $l(x) = \log\left(1 + \exp(-x)\right)$ be the logistic function, we have $l^\prime(x) = -1/(1 + \exp(x)) < 0$. 
Let $f(\Wv, \Xv) = F_1(\Wv, \Xv) - F_{-1}(\Wv, \Xv)$.
The loss on single input $(\Xv, y)$ is defined as $L(\Wv, \Xv, y) = l(yf(\Wv,\xv))$. Let $L_i = L(\Wv, \Xv_i, y_i)$, the training objective is 
\begin{align*}
    L = \frac{1}{n}\sum_{i\in[n]}L_i.
\end{align*}
