# Supplementary material for: On the Optimization and Generalization of Two-layer Transformers with Sign Gradient Descent
Source: arXiv:2410.04870 source file (2025-03-02)
Supplement: Supplementary file 5 [file prelim_experiments.tex]

\newpage
\section{Key questions and empirical analysis}

This section is important because it talks about the motivation and goal of our work. 
In this work, generally speaking, we try to analyze the benign overfitting behavior in Transformers with Adam. 
Our contribution is:
\begin{enumerate}
    \iffalse
    \item Transformer is important. Under the same data model, given any optimizer (or one of them), Transformers can tolerate more noisy data than CNNs/Linear models. The point is to show Transformers may tolerate more noises in data. (Roughly, CNN\&TF + GD with tunable noise)
    \item Adam is important (in Transformers). Prior work showed that Adam is not as good as GD when there are many noisy entries in data. The point is comparing between Transformers and CNNs with both trained using Adam. (Roughly, CNN\&TF + Adam)
    \item We do not compare Transformers with any other models. Just give the dynamics and talk about how Transformers learn the features and/or noises under different data models (with Adam). The dynamics of attention weights with Adam will be rich and different compared with CNNs. This is similar to ideas in~\citep{cao2022benign} but with Transformers and Adam. (Roughly, TF + Adam with tunable noise)
    \fi
    \item We compare the behaviour of different optimizers on Transformers under one fixed data model, which is similar to ideas and results in~\citep{zou2021understanding}  (Roughly, TF + Adam\&GD). 
    In this data model, GD falls into benign overfitting and Adam falls into harmful overfitting.
    \item The contribution is: 1. we state the behavior in Transformers
    \item 2. we give a different insight when optimized with Adam, the fast convergence of attention weights.
\end{enumerate}

Some concerns are
\begin{enumerate}
    \item When using GD, the analysis of Transformers would be very similar to CNNs. The learning of attention weights are far behind value parameters.
    \item \textbf{The point is: How to show/distinguish our contribution?} If we try to compare two models, the perspectives are: 1) \textbf{accuracy}, which is the most persuasive. For example, under the same SNR and optimizer, one model is in the benign overfitting regime, while the other model is in the noise memorization regime. 2) \textbf{mechanism}, which is subtle and delicate. For example, under the same SNR and optimizer, both models are in benign overfitting regime but the reasons are different. For example, the parameters of one model (such as CNN) learn faster towards the direction of noise than the direction of feature~\citep{cao2022benign}. However, the other model (such as ideal Transformers) learns this by attention mechanism, i.e., the attention weights are the main reasons. 
    We talk more about this in subsection~\ref{sec:empirial-accuracy-comparison}.
    \item What models should we use? The difference in architecture may lead to different empirical results, difficulty of analysis, and something intrinsic (but less likely), thus different conclusions. We talk more about this in subsection~\ref{sec:arch-choice}.
    \item How to simplify Adam to make it easy to analyze? See discussion in section~\ref{sec:empirial-training-dynamics}.
\end{enumerate}

\subsection{Empirical accuracy comparison}
\label{sec:empirial-accuracy-comparison}
\subsubsection{Standard accuracy comparison}
Given any optimizer and model, we focus on the test loss trained with a long enough time across different SNR. 

\paragraph{Hyperparameters}
We consider different optimizers, i.e., GD, Adam($\beta_1=0.9, \beta_2=0.999$), GD(+m)($\beta_1=0.9$), Adam(-m)($\beta_1=0, \beta_2=0.999$), and sign GD($\beta_1=0, \beta_2=0$), with fixed learning rate on different architectures: 1) activation functions, 2) positions of activation function, 3) attention type. The most practical Transformer model uses linear activation and softmax attention. See details about model definitions in section~\ref{sec:arch-choice}.

We use $d = m_k = 400, n = 100, m_v = 20$, since this set of hyperparameters is representative. 
We use initialization variance $\sigma_0 = 0.1 / \sqrt{d}$ and learning rate (dependent on optimizers) as small as as possible because we found this would lead to small variance. To further reduce variance, we run 10 times and average the result for each point in a curve. We also consistently train 400 epochs with full batch size, to ensure each run is trained long enough. 

By the way, if we use a slightly large initialization std like $1 / \sqrt{d}$, it would cause big variance even if in large SNR regime, shown in Fig.~\ref{fig:loss-snr-large-initialization}.

\paragraph{Changing SNR.}
Recall SNR is defined as $\norm{\muv} / \sigma_p\sqrt{d}$. We follow the experiments in~\citep{cao2022benign} that we change SNR by changing feature magnitude and fixing noise level $\sigma_p = 1$. This is more appropriate (compared with changing noise magnitude) in the sense that we expect the range of valid learning rate to stablize training would not vary too much as SNR changes since the feature only has one real entry. The range of SNR used is typically $[0.1, 1]$. A caveat is that we use fixed ``random'' data(seed=3407) between multiple runs, which can be improved by different random data across runs.

\paragraph{Summary of observation.}

Fig.~\ref{fig:loss-snr-softmax-attn},\ref{fig:loss-snr-fix-attention},\ref{fig:loss-snr-linear-attention} show the test loss of different models trained with different optimizers under different SNRs.
There are some observations:
\begin{enumerate}
    \item Whether fix $\Wv_Q,\Wv_K$ or not doesn't have a big influence on GD($\pm$m). This means 1) the attention is trained but not helpful for GD to perform this task, or 2) the attention is barely trained compared with value parameters, thus only contribute a little
    (The mechanistic reason why they are indistinguishable is not explored in this section).
    This might suggests that the mechanism for Transformers and CNNs is similar, thus the analysis is probably incremental. In summary, focus on GD may be less contributed.
    \item The role of Adam (or adaptive gradient) on attention weights (the learning of $\Wv_Q,\Wv_K$) is not too clear, since we cannot see enable attention weights to learning makes it better consistently on given model and optimizer. In other words, Adam, Adam(-m), and sign GD behaves different. This can be clearly seen in Fig.~\ref{fig:loss-snr-fix-attention}. Also, the evidence on large SNR is provided in Fig.~\ref{fig:loss-snr-large-initialization}. But there is one invariant point: as SNR gets large, the model with fixed $\Wv_Q,\Wv_K$ outperforms than learning $\Wv_Q,\Wv_K$.
    However, the behaviour of GD and GD(+m) are consistent on this task.
    \item When we use model with linear attention, we can see it is not the case that GD left other optimizers far behind at any time. When using ReLU$^3$, sign GD and Adam(-m) are similar, three of the rest optimizers are similar. When using linear activation, GD($\pm$m) outperform than others, Adam(-m) is the worst.
\end{enumerate}

\begin{figure}
    \centering
    \includegraphics[width=1.0\textwidth]{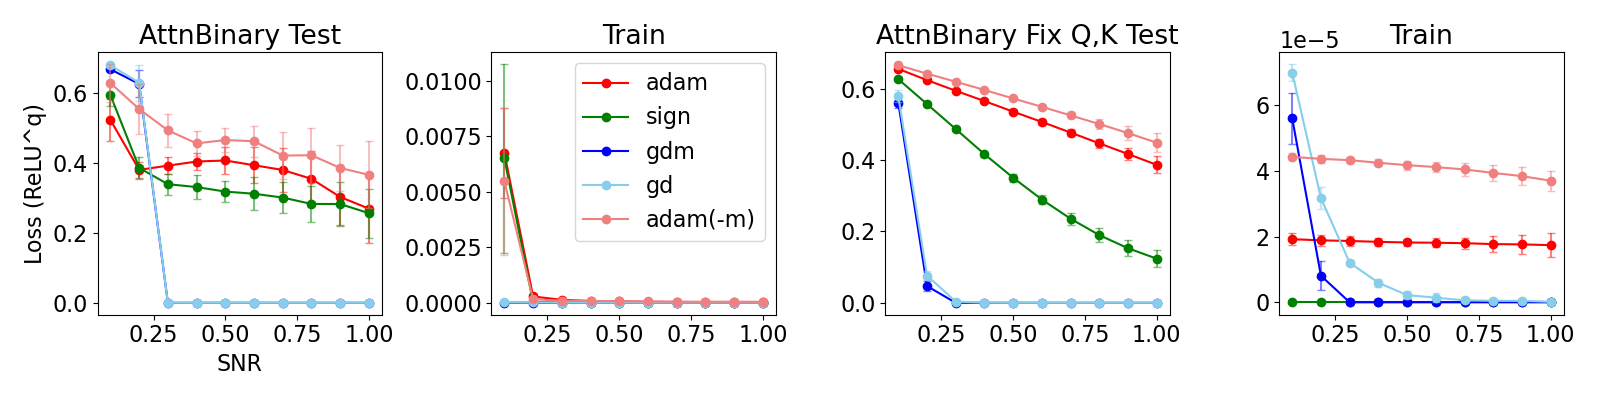}
    \includegraphics[width=1.0\textwidth]{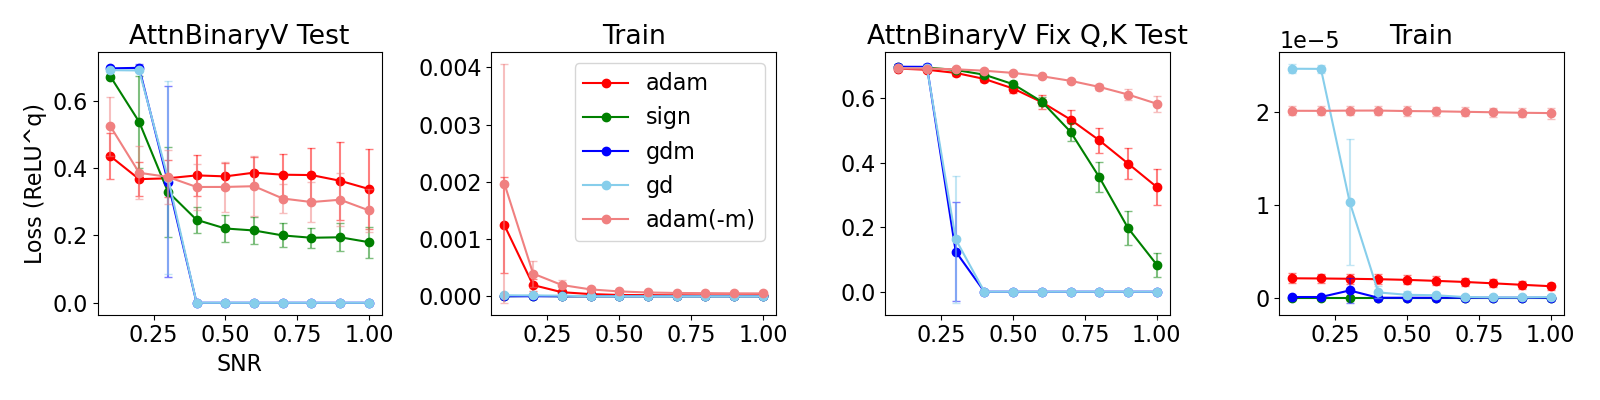}
    \includegraphics[width=1.0\textwidth]{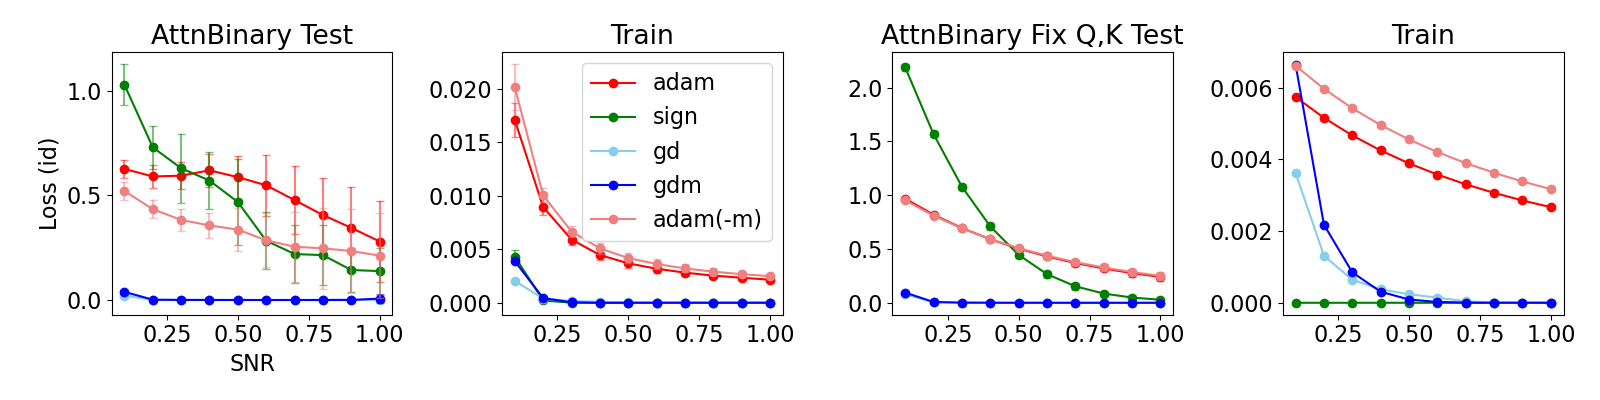}
    \caption{
    Test loss versus SNR, with all optimizers on $\mathsf{AttnBinary}$/$\mathsf{AttnBinaryV}$ with softmax attention. $\sigma_0 = 0.1 / \sqrt{d}$.
    Line 1 shows results on $\mathsf{AttnBinary}$ with ReLU$^3$.
    Line 2 shows results on $\mathsf{AttnBinaryV}$ with ReLU$^3$.
    Line 3 shows results on $\mathsf{AttnBinary}$ with linear activation.
    SNR ranges from 0.1 to 1.0. 
    learning rates: GD($\eta = 1$), Adam($\eta = 1e-3$), GD(+m)($\eta = 0.05$), sign GD($\eta = 1e-3$), Adam(-m)($\eta = 1e-3$).
    }
    \label{fig:loss-snr-softmax-attn}
\end{figure}

\begin{figure}
    \centering
    \includegraphics[width=1.0\textwidth]{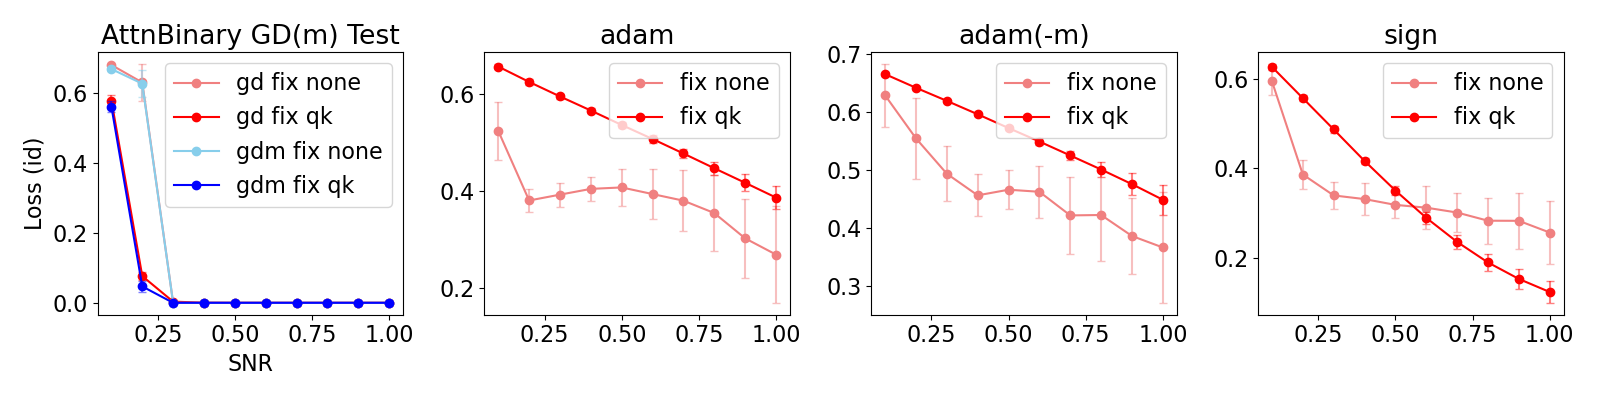}
    \includegraphics[width=1.0\textwidth]{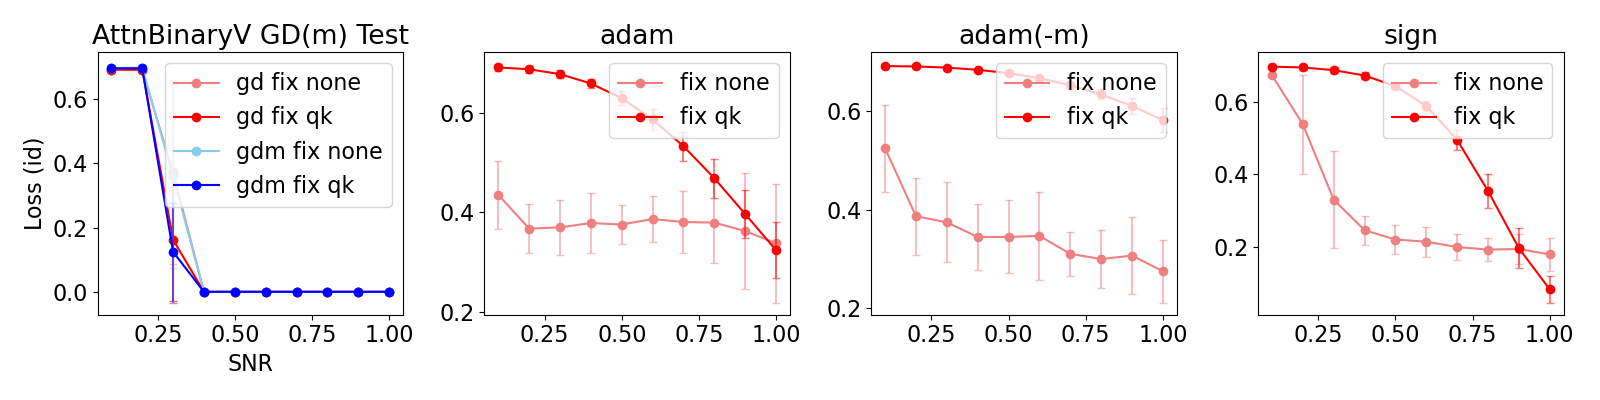}
    \includegraphics[width=1.0\textwidth]{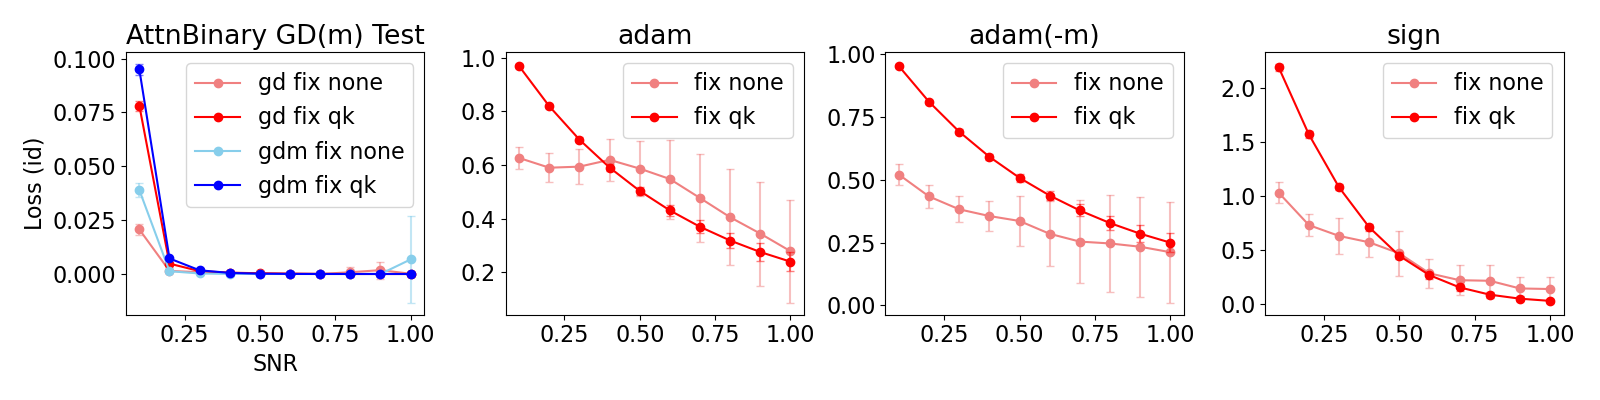}
    \caption{
    Test loss versus SNR, with all optimizers on $\mathsf{AttnBinary}$/$\mathsf{AttnBinaryV}$ with softmax attention. $\sigma_0 = 0.1 / \sqrt{d}$.
    Line 1 shows results on $\mathsf{AttnBinary}$ with ReLU$^3$.
    Line 2 shows results on $\mathsf{AttnBinaryV}$ with ReLU$^3$.
    Line 3 shows results on $\mathsf{AttnBinary}$ with linear activation.
    SNR ranges from 0.1 to 1.0. 
    learning rates: GD($\eta = 1$), Adam($\eta = 1e-3$), GD(+m)($\eta = 0.05$), sign GD($\eta = 1e-3$), Adam(-m)($\eta = 1e-3$).
    }
    \label{fig:loss-snr-fix-attention}
\end{figure}

\begin{figure}
    \centering
    \includegraphics[width=1.0\textwidth]{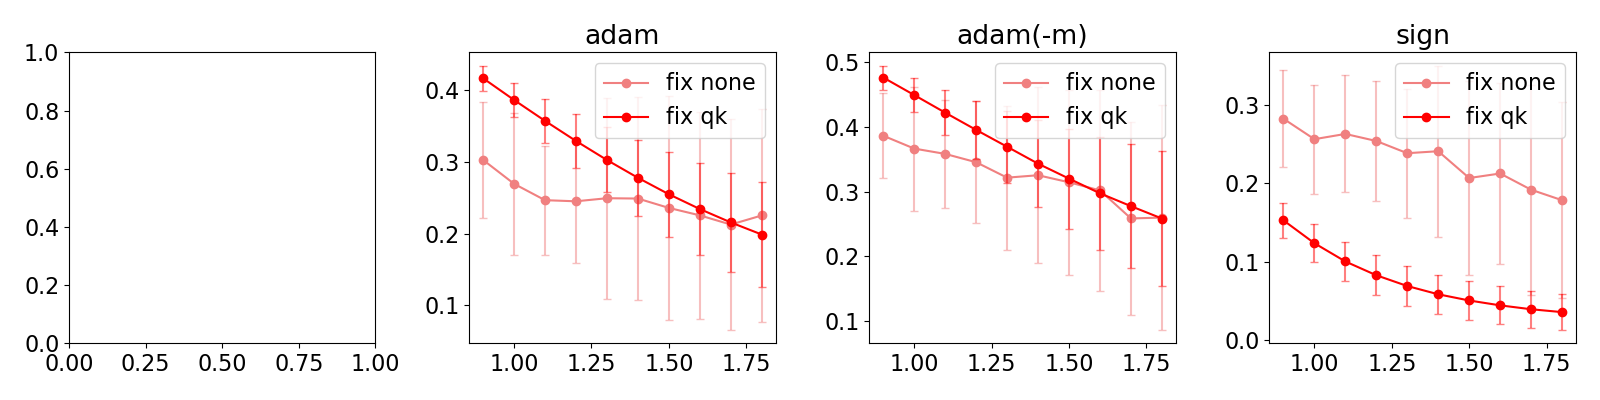}
    \includegraphics[width=1.0\textwidth]{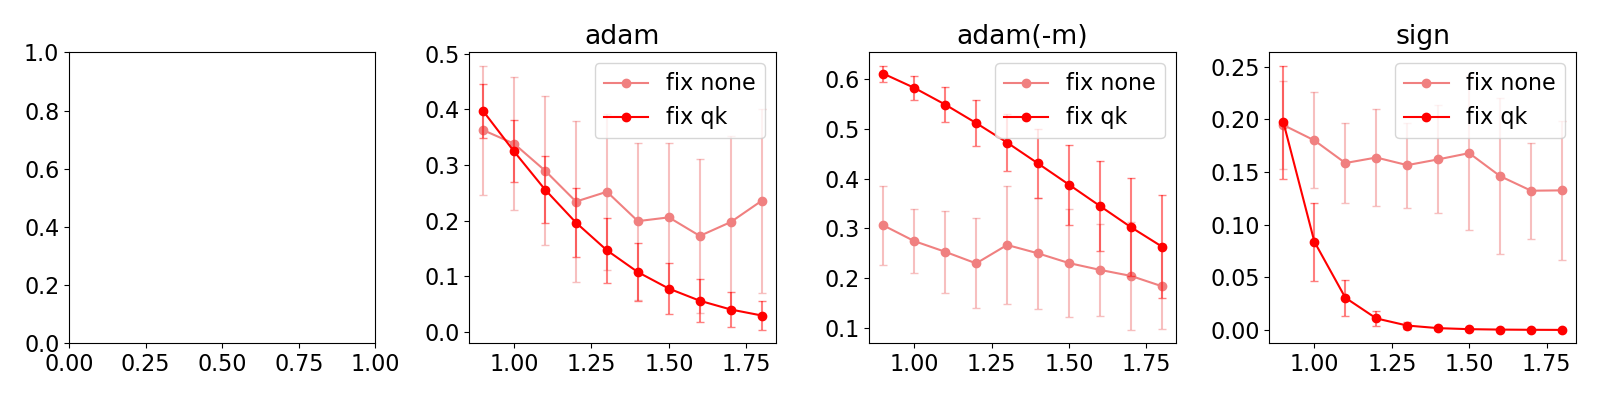}
    \includegraphics[width=1.0\textwidth]{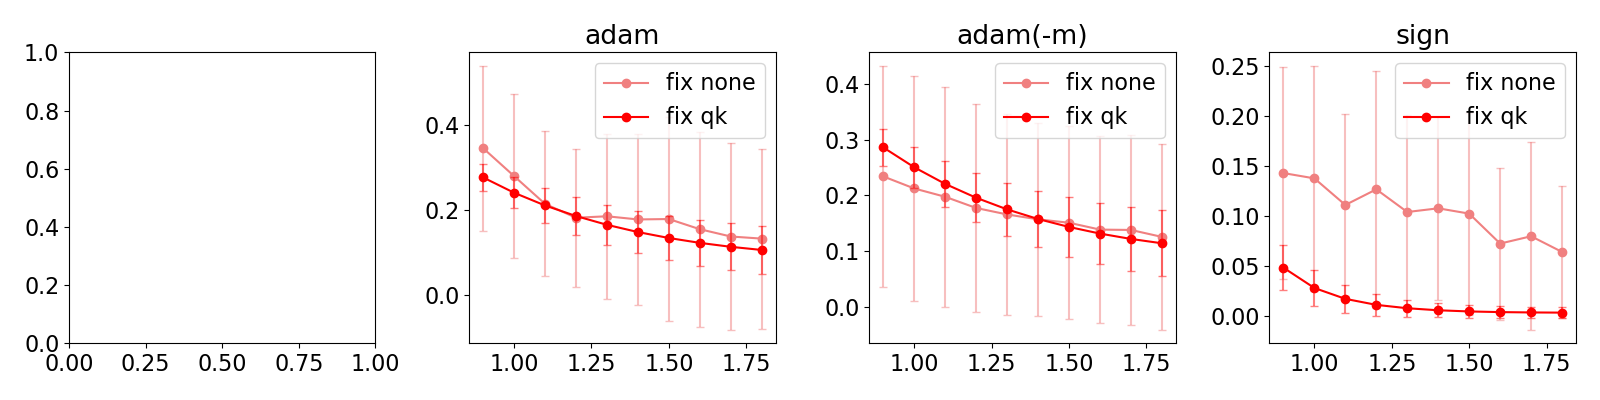}
    \caption{
    Test loss versus (large) SNR, with all optimizers on $\mathsf{AttnBinary}$/$\mathsf{AttnBinaryV}$ with softmax attention. $\sigma_0 = 0.1 / \sqrt{d}$.
    Line 1 shows results on $\mathsf{AttnBinary}$ with ReLU$^3$.
    Line 2 shows results on $\mathsf{AttnBinaryV}$ with ReLU$^3$.
    Line 3 shows results on $\mathsf{AttnBinary}$ with linear activation.
    SNR ranges from 0.9 to 1.8. 
    learning rates: Adam($\eta = 1e-3$), sign GD($\eta = 1e-3$), Adam(-m)($\eta = 1e-3$).
    }
    \label{fig:loss-snr-large-snr}
\end{figure}

\begin{figure}
    \centering
    \includegraphics[width=1.0\textwidth]{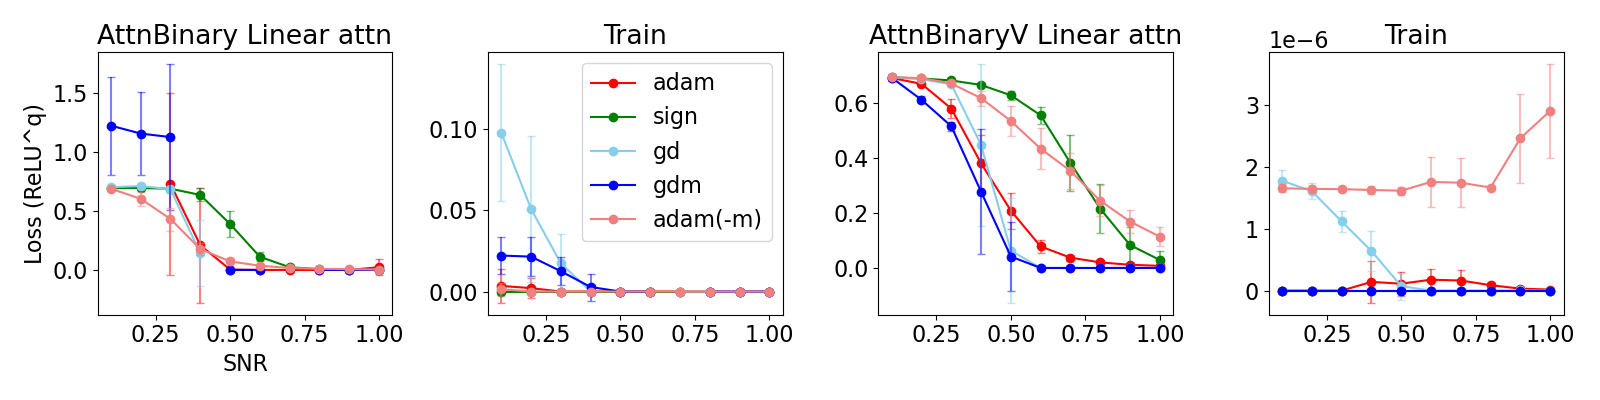}
    \includegraphics[width=1.0\textwidth]{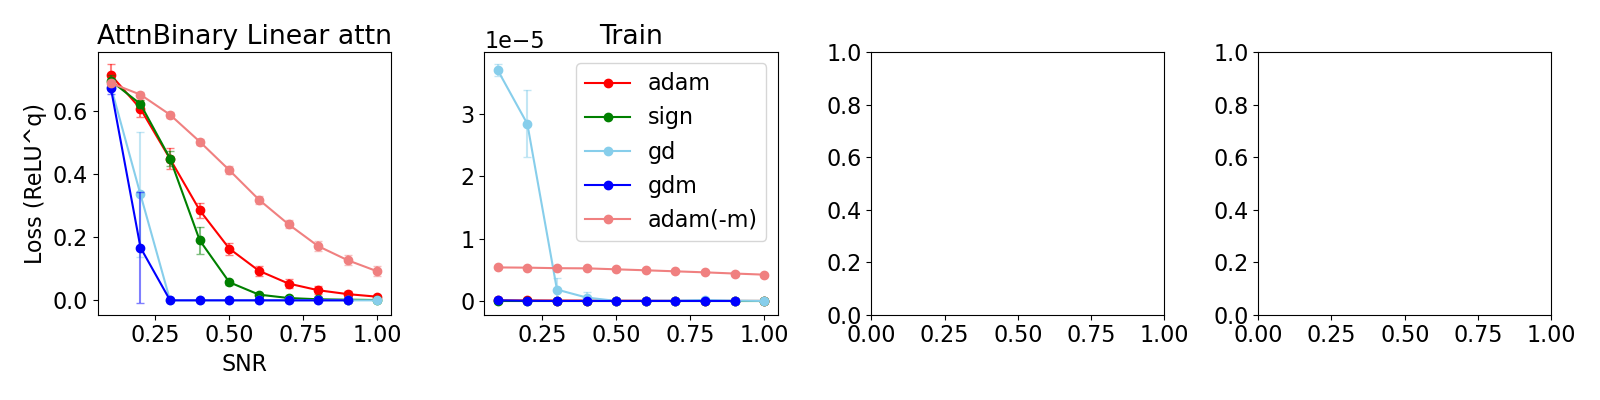}
    \caption{Test loss versus SNR, with all optimizers on AttnBinary/AttnBinaryV with linear attention. 
    Line 1 uses ReLU$^3$, $\sigma_0 = 0.1 / \sqrt{d}$, GD($\eta = 1$), Adam($\eta = 5e-4$), sign GD($\eta = 5e-4$), GD(+m)($\eta = 0.05$), Adam(-m)($\eta = 5e-4$), .
    Line 2 uses linear activation, $\sigma_0 = 0.1 / \sqrt{d}$, same lr as line 1.
    SNR ranges from 0.1 to 1.0. 
    }
    \label{fig:loss-snr-linear-attention}
\end{figure}

\begin{figure}
    \centering
    \includegraphics[width=1.0\textwidth]{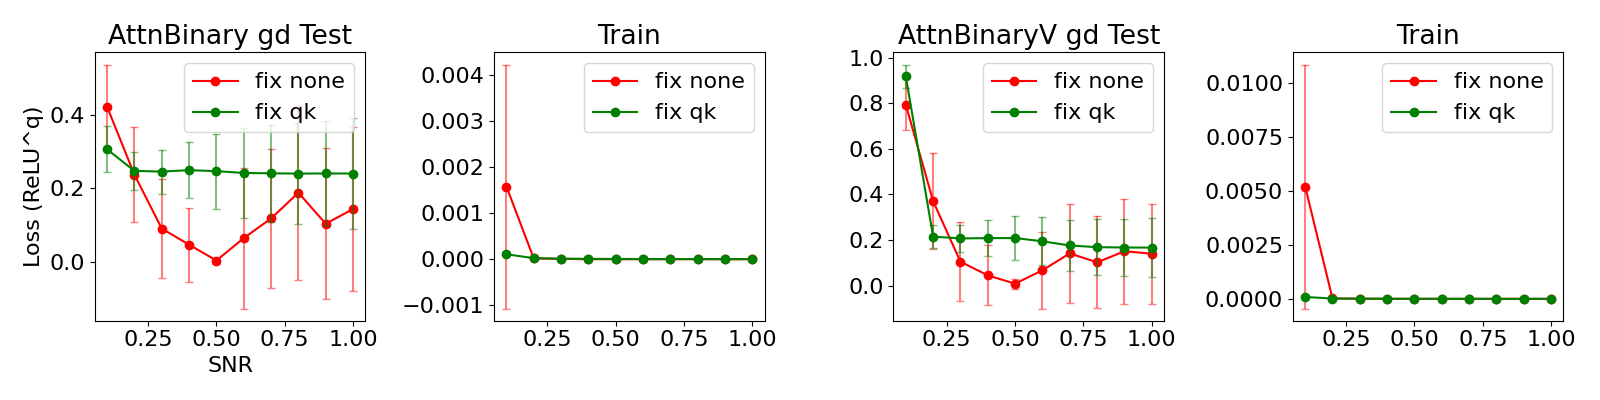}
    \includegraphics[width=1.0\textwidth]{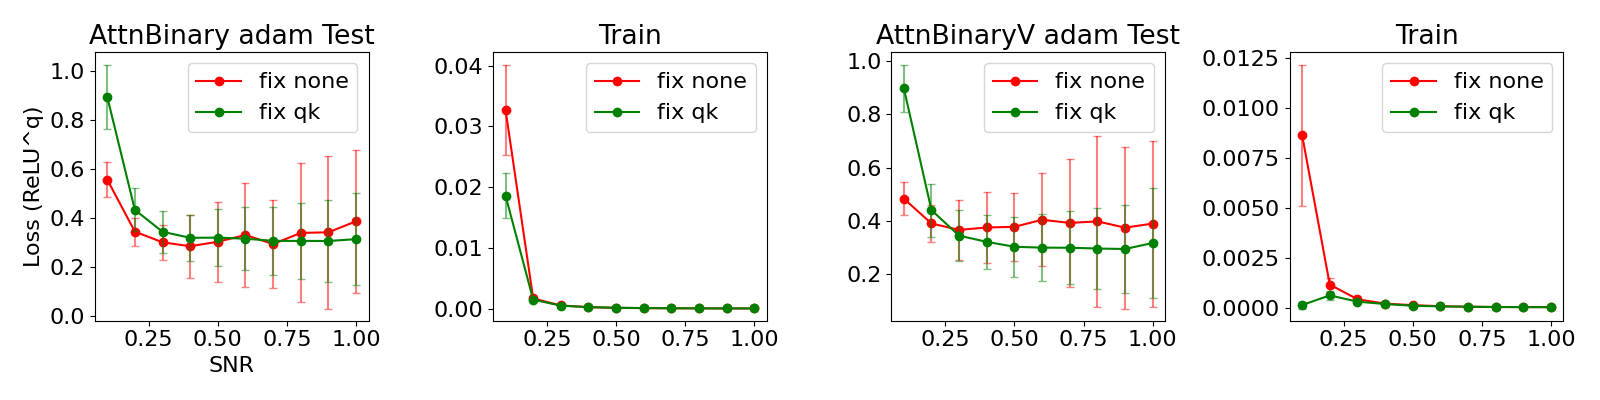}
    \caption{Test loss versus SNR, curse of with large initialization, with AttnBinary/AttnBinaryV + ReLU$^3$.
    Line 1 uses $\sigma_0 = 1 / \sqrt{d}$, GD($\eta=1$), SNR ranging from 0.1 to 1.0. 
    Line 2 uses $\sigma_0 = 1 / \sqrt{d}$, Adam($\eta = 1e-3$), SNR ranging from 0.1 to 1.0. 
    }
    \label{fig:loss-snr-large-initialization}
\end{figure}

\subsubsection{Specific accuracy comparison related to dynamics experiments}
TODO

\subsection{Emprical training dynamics}
\label{sec:empirial-training-dynamics}
In this section, we show the training dynamics of adaptive optimizers under fixed data model. We aim to 1) grasp the key features in dynamics of Adam, and 2) simiplify Adam to a optimizer easier to analyze.

\subsubsection{Middle-level quantities}
In this section, we care about quantities listed below
\begin{itemize}
    \item 0-1 loss
    \item cross entropy loss
    \item attention weights (a $2\times2$ matrix with sum of each row equal to 1)
    \item feature learning and noise memorization quantity, i.e., value inner product in the context of Transformers, defined as $\max_{j,r} \abs{\gamma_{j,r}} = \max_{j,r} \abs{\langle \wv_{V,j,r}, \muv\rangle}$ and $\max_{j,r} \abs{\rho_{j,r,i}} = \max_{j,r} \abs{\langle \wv_{V,j,r}, \xiv_i\rangle}$ for all $i\in[n]$.
    \item relevant quantities for query and key. Formally, we care about $\max_{s}  \abs{\langle \wv_{Q,s}, \muv\rangle}, \max_{s}  \abs{\langle \wv_{Q,s}, \xiv_i\rangle}, \max_{s}  \abs{\langle \wv_{K,s}, \muv\rangle}, \max_{s} \abs{\langle \wv_{K,s}, \xiv_i\rangle}$ for all $i\in[n]$.
\end{itemize}

\paragraph{Hyperparameters}
We consider different optimizers, i.e., Adam($\beta_1=0.9, \beta_2=0.999$), Adam(-m)($\beta_1=0, \beta_2=0.999$), signGD1(using Adam with $\beta_1=0, \beta_2=0$), signGD2 and normalized GD with fixed learning rate. $\epsilon$ is set to 1e-8 in default. 
Notably, signGD1 can be seen as a smooth verision of real signGD (signGD2), as the gradient magnitude has a sigmoid-like shape instead of hard step function.
Actually, it is hard to compare between these optimizers fairly with same $\eta$ since it may not imply same effective learning rate, but we don't care too much about this here.
We consider different architectures: 1) activation functions, and 2) positions of activation function. The most practical Transformer model uses linear activation and softmax attention. See details about model definitions in section~\ref{sec:arch-choice}.

We use $d = m_k = 2000, n = 100, m_v = 20$. We use initialization variance $\sigma_0 = 0.1 / \sqrt{d}$ and learning rate as small as possible (but able to converge) to see more fine-grained dynamics, where we do this by assuming learning rate only slows down everything but not change the regime.
In every setting, we run 3 random models. We consistently train 400/700 epochs with full batch size, to ensure each run is trained long enough. 

We use data model with hyperparameters: $\text{SNR}=1, \sigma_p=1/\sqrt{d}$.

\paragraph{Summary of Observation}
Fig.~\ref{fig:dynamics-AttnBinary-linear-1},\ref{fig:dynamics-AttnBinary-linear-2},\ref{fig:dynamics-AttnBinary-ReLU3-1},\ref{fig:dynamics-AttnBinary-ReLU3-2},\ref{fig:dynamics-AttnBinaryV-ReLU3-1},\ref{fig:dynamics-AttnBinaryV-ReLU3-2},\ref{fig:dynamics-normgd} show the dynamics on different models trained with different optimizers.
There are some observations:
\begin{itemize}
    \item Generally, the behavior in terms of test loss, feature/noise learning (i.e., value inner product), and query \& key inner product are similar between Adam and sign GD. Some subtle difference are stated below.
    \item With small learning rate, test loss across different runs have less variance while variance increases with large learning rate. 
    The large variance is led by the attention mechanism. When only one sample attends to feature, test loss decreases a lot compared with the case where none of training samples attend to feature. The difference is especially obvious when the number of samples attending to features is quite small, e.g., signGD1 generalizes in Fig.~\ref{fig:dynamics-AttnBinary-linear-1}. This can also explain the large variance of trained attention models in figures of section~\ref{sec:empirial-accuracy-comparison}.
    \item Beyond the variance, some observations are: With linear activation, \textcolor{red}{when there exists some training samples attending to feature}, feature grows faster with sign GD than Adam. So does noise, which can be clearly seen in Fig.~\ref{fig:dynamics-AttnBinary-linear-2}. After check, this is identified by the small magnitude of query/key parameters gradients ($\lesssim$ 1e-8) compared with the optimzier hyperparameter $\epsilon$ of 1e-8.
    \item The query and the key vectors: the trend of increase cannot by simply summarized to some conclusion about which is generally faster than the other. In linear activation setting, Adam and signGD2 resemble while there is a large difference in magnitude in other model settings.
    \item With linear activation, all value inner products grow (sine ReLU has a filter role). 
    \item Normalized GD behaves differently from adaptive optimizers. See Fig.~\ref{fig:dynamics-normgd}.
\end{itemize}

\begin{figure}
    \centering
    \includegraphics[width=0.9\textwidth]{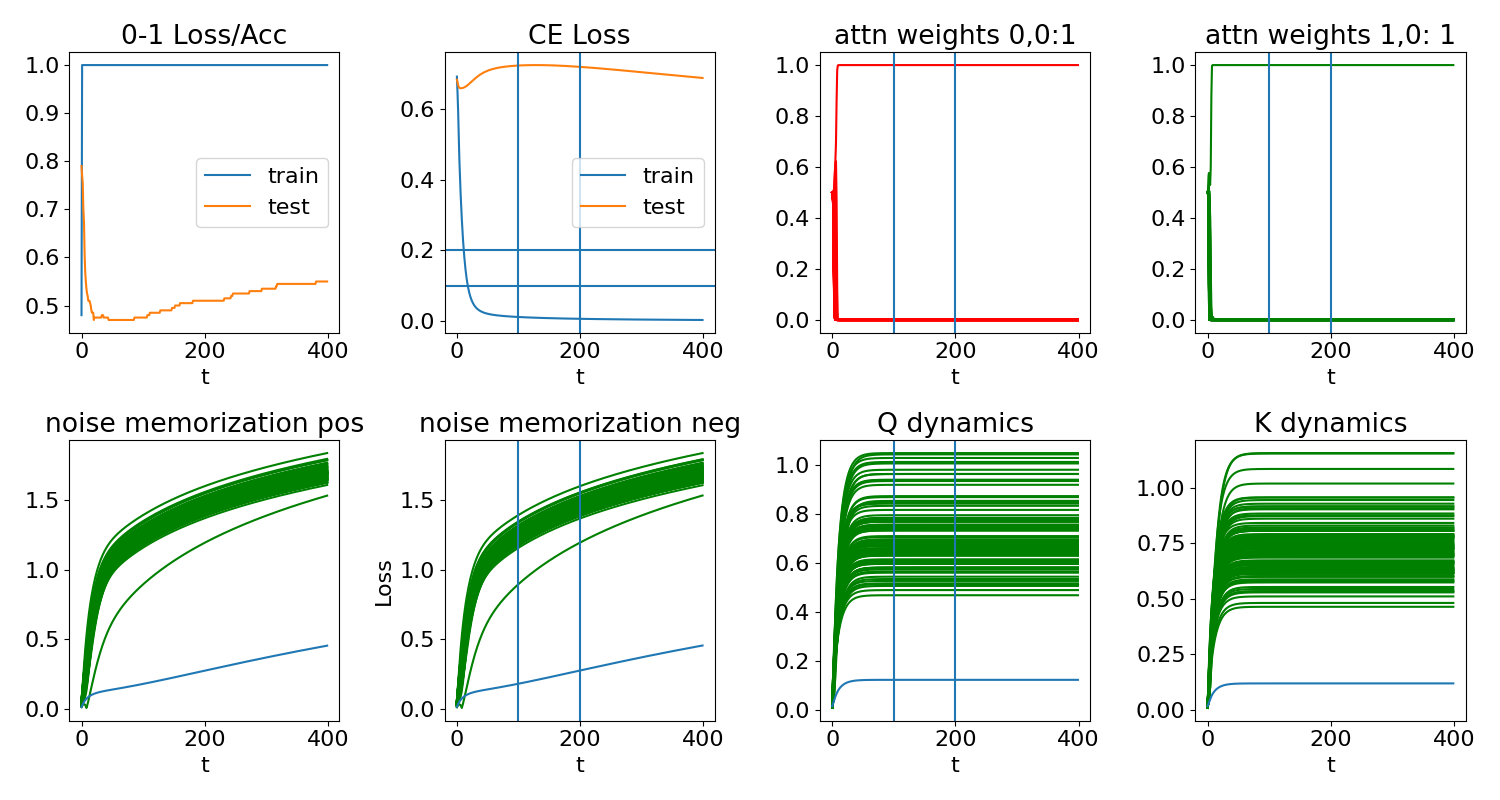}
    \includegraphics[width=0.9\textwidth]{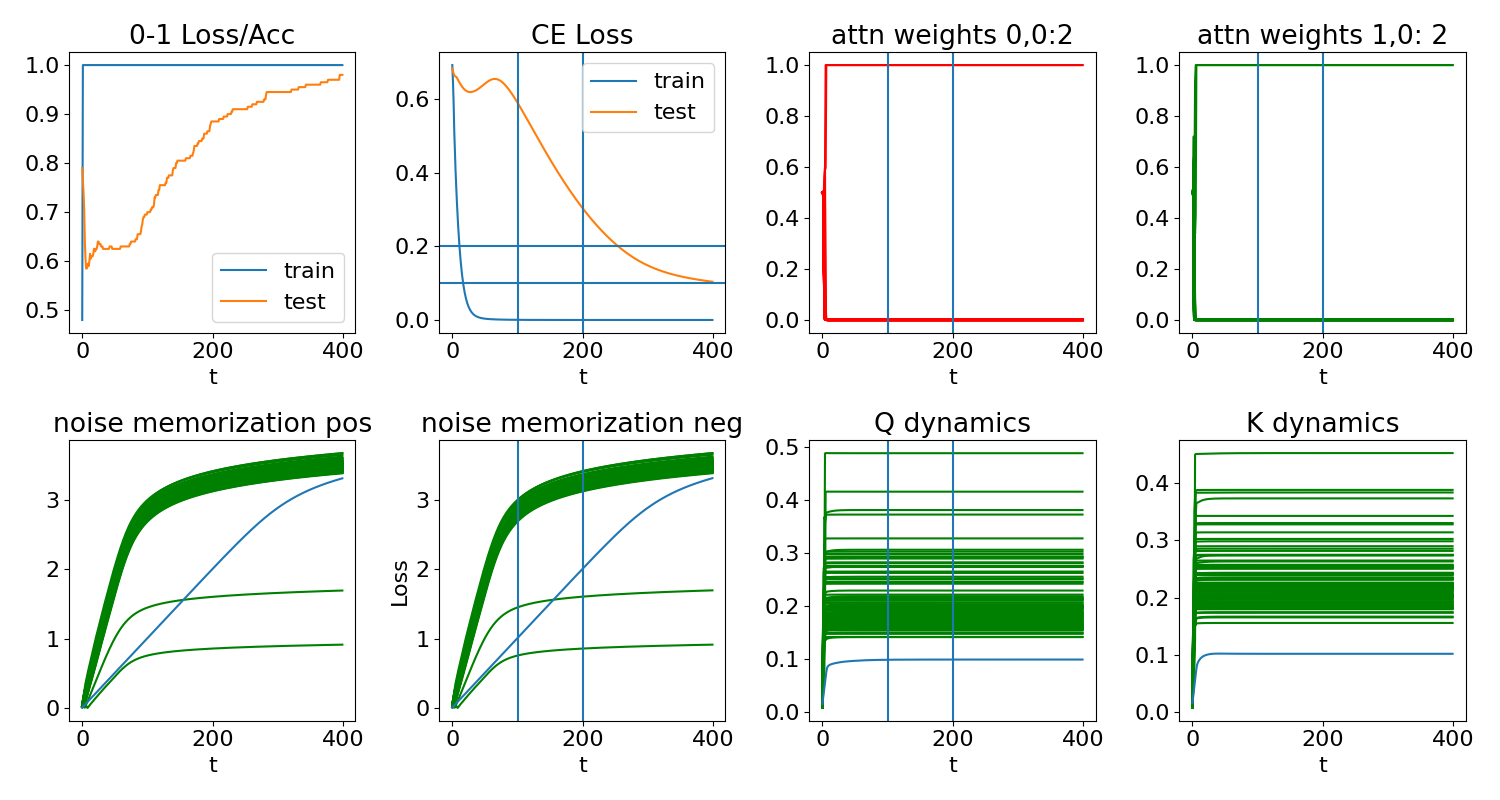}
    \includegraphics[width=0.9\textwidth]{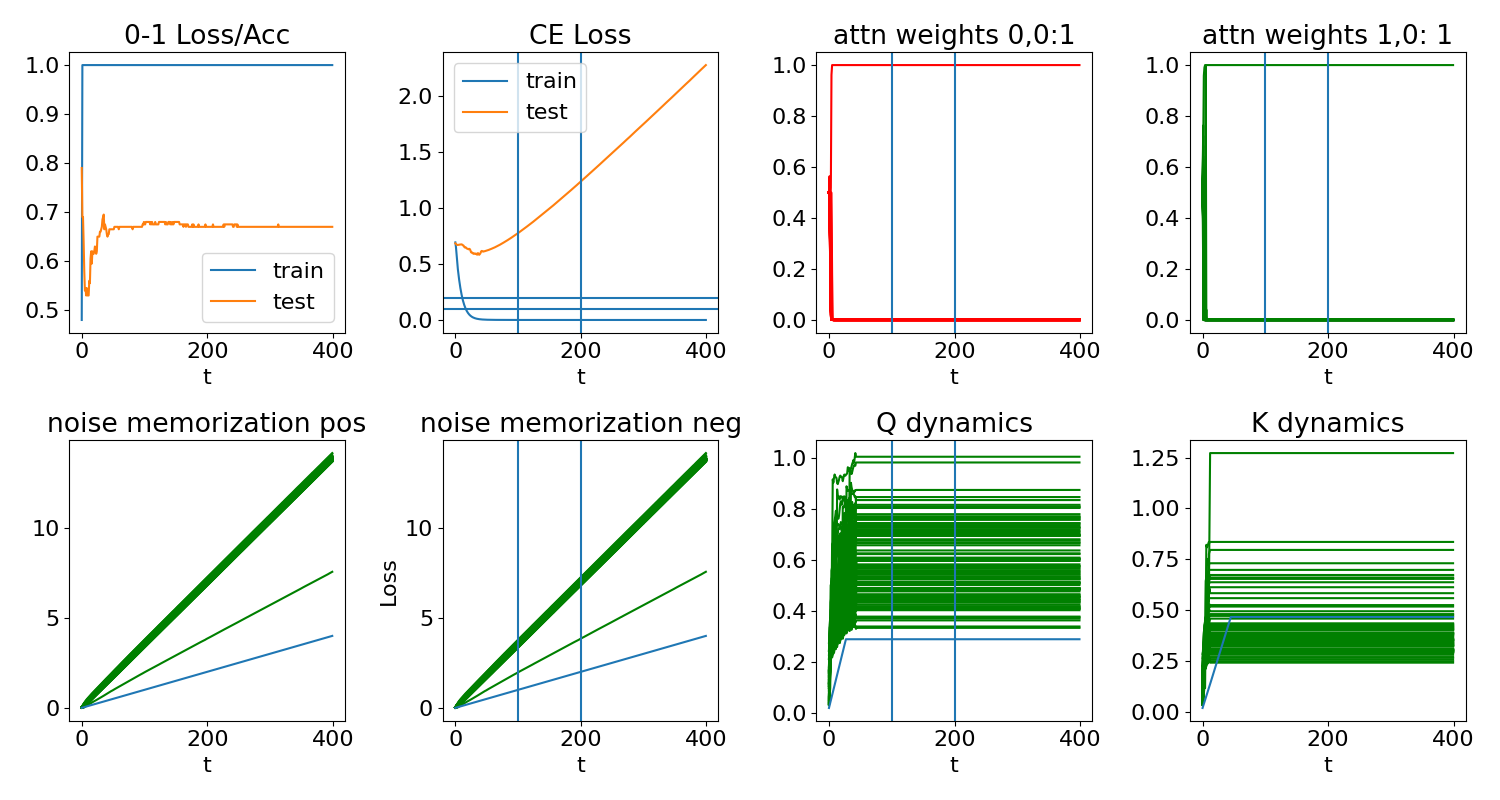}
    \caption{Dynamics, with AttnBinary + linear activation.
    Line 1: Adam($\eta = 1e-2$). Line 2: signGD1($\eta = 1e-2$). 
    Line 3: signGD2($\eta = 1e-2$).
    }
    \label{fig:dynamics-AttnBinary-linear-1}
\end{figure}

\begin{figure}
    \centering
    \includegraphics[width=0.9\textwidth]{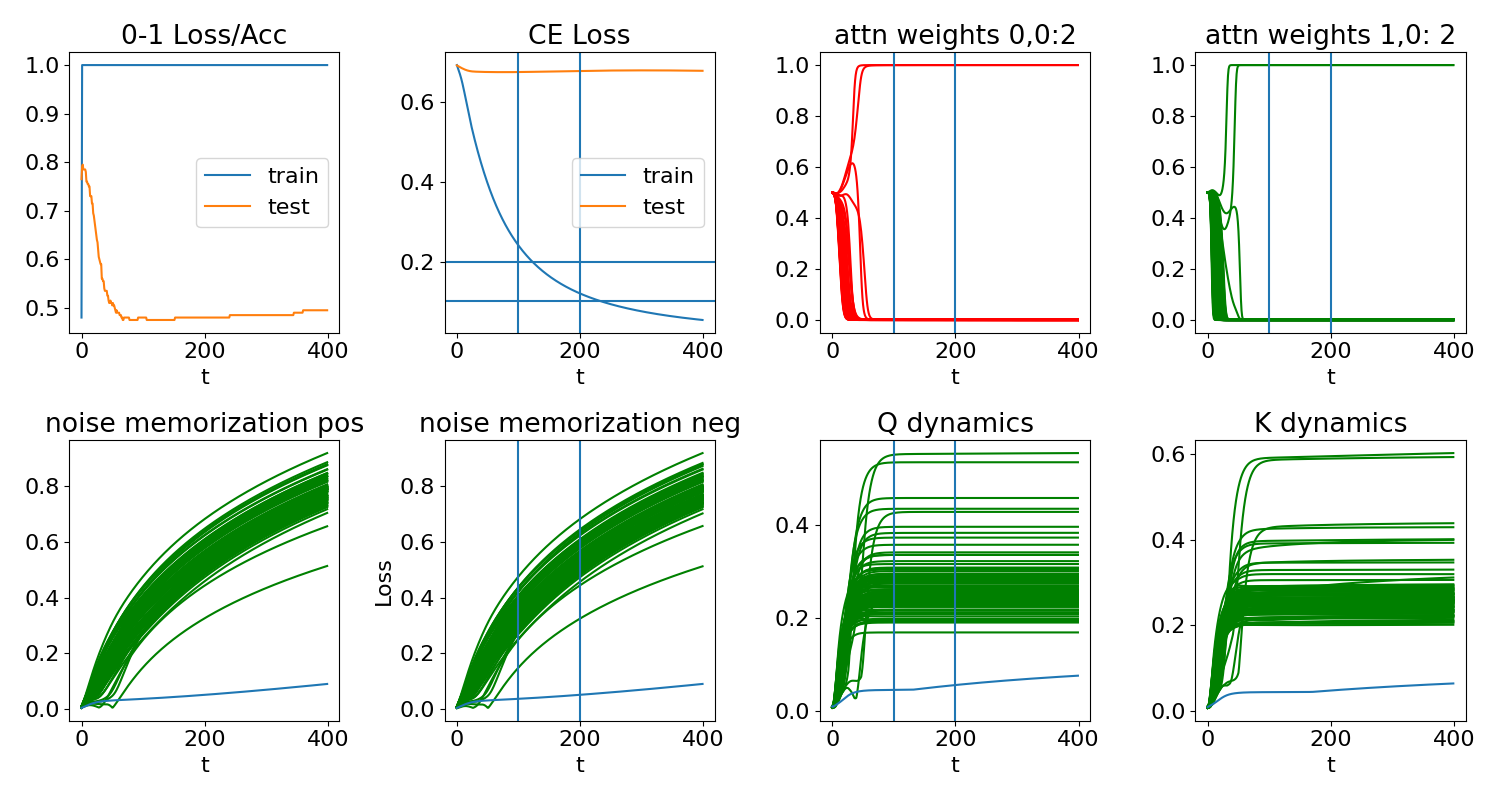}
    \includegraphics[width=0.9\textwidth]{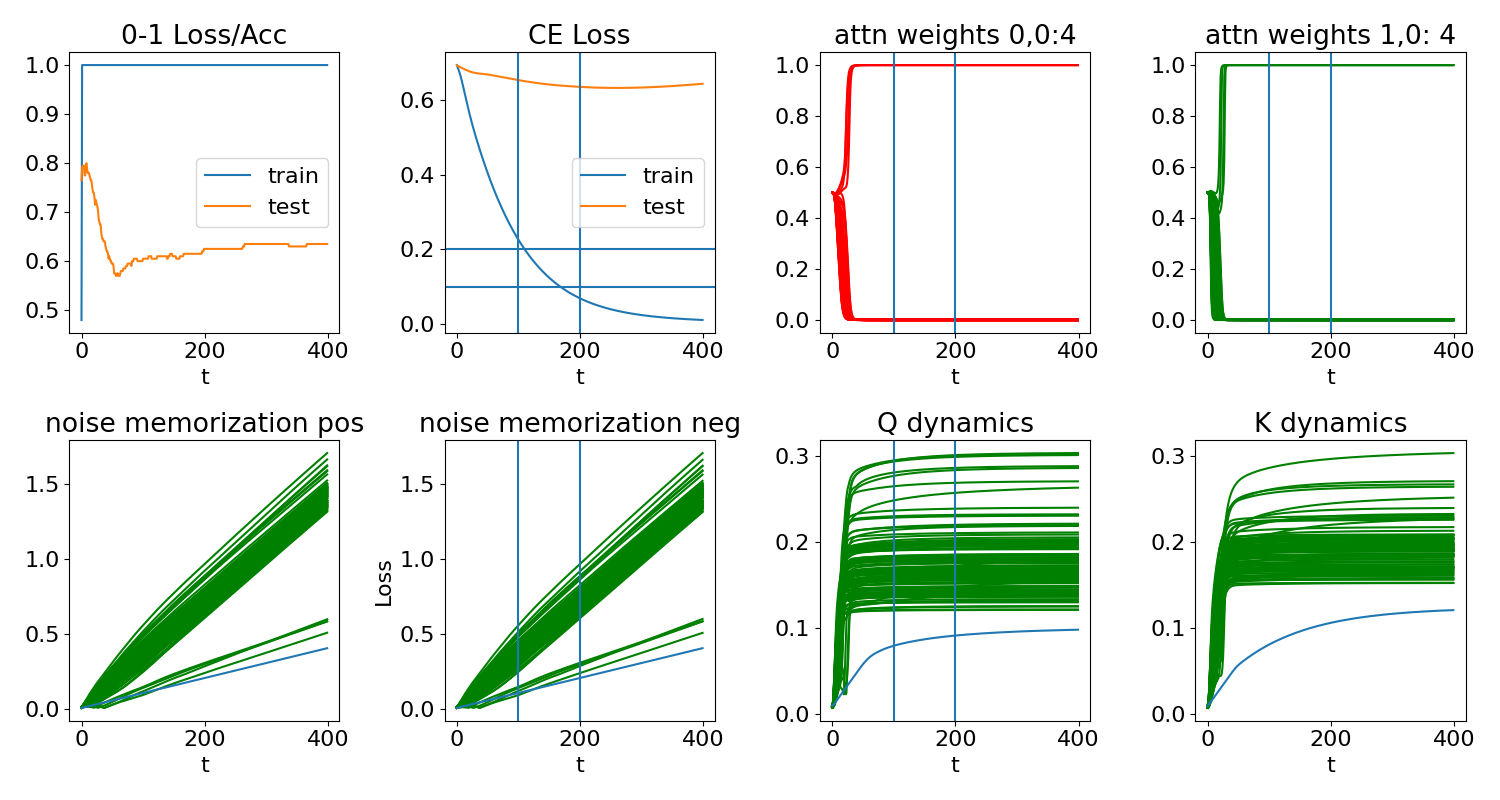}
    \includegraphics[width=0.9\textwidth]{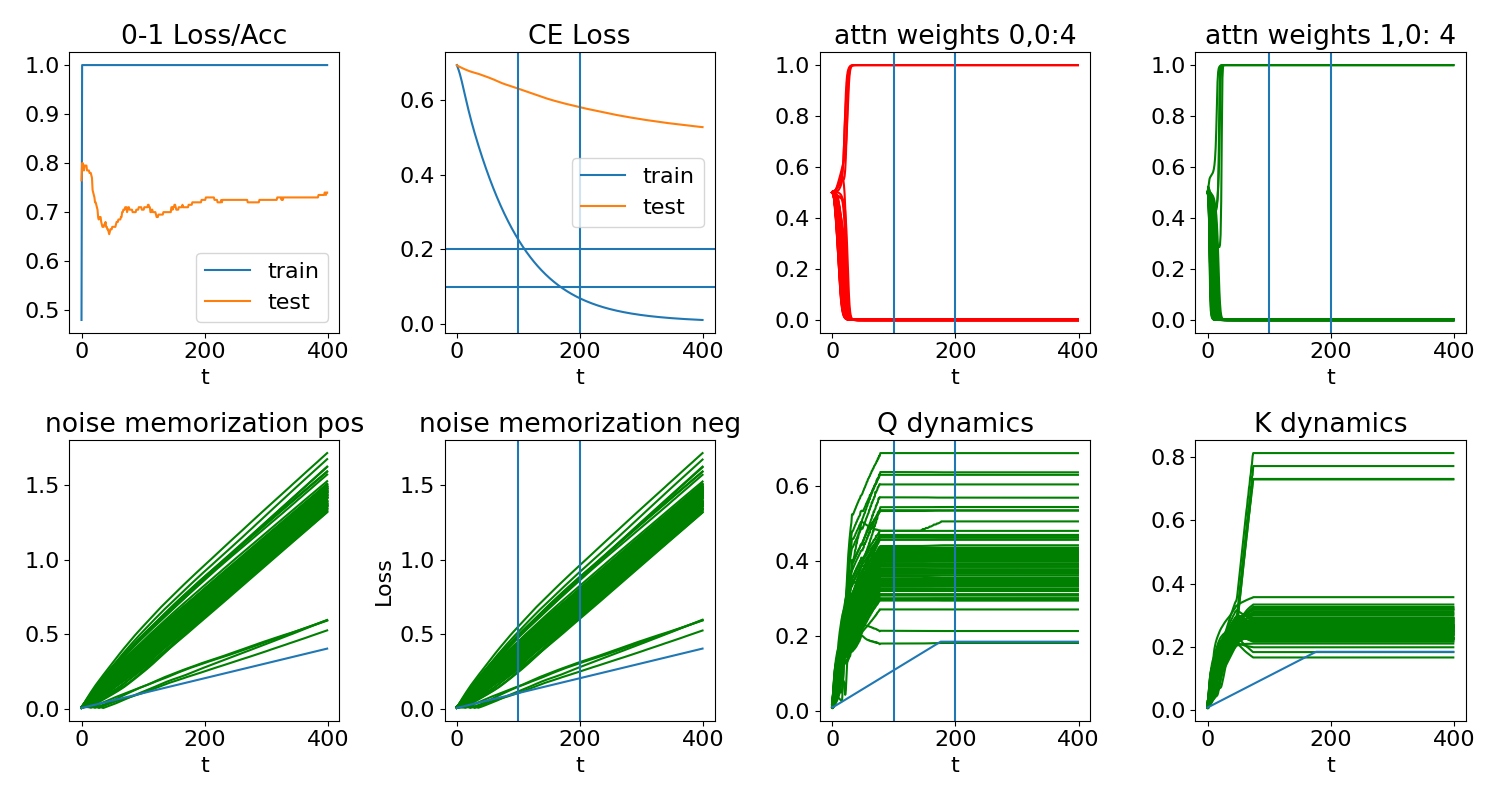}
    \caption{Dynamics, with AttnBinary + linear activation.
    Line 1: Adam($\eta = 1e-3$). Line 2: signGD1($\eta = 1e-3$). 
    Line 3: signGD2($\eta = 1e-3$).
    }
    \label{fig:dynamics-AttnBinary-linear-2}
\end{figure}

\begin{figure}
    \centering
    \includegraphics[width=0.9\textwidth]{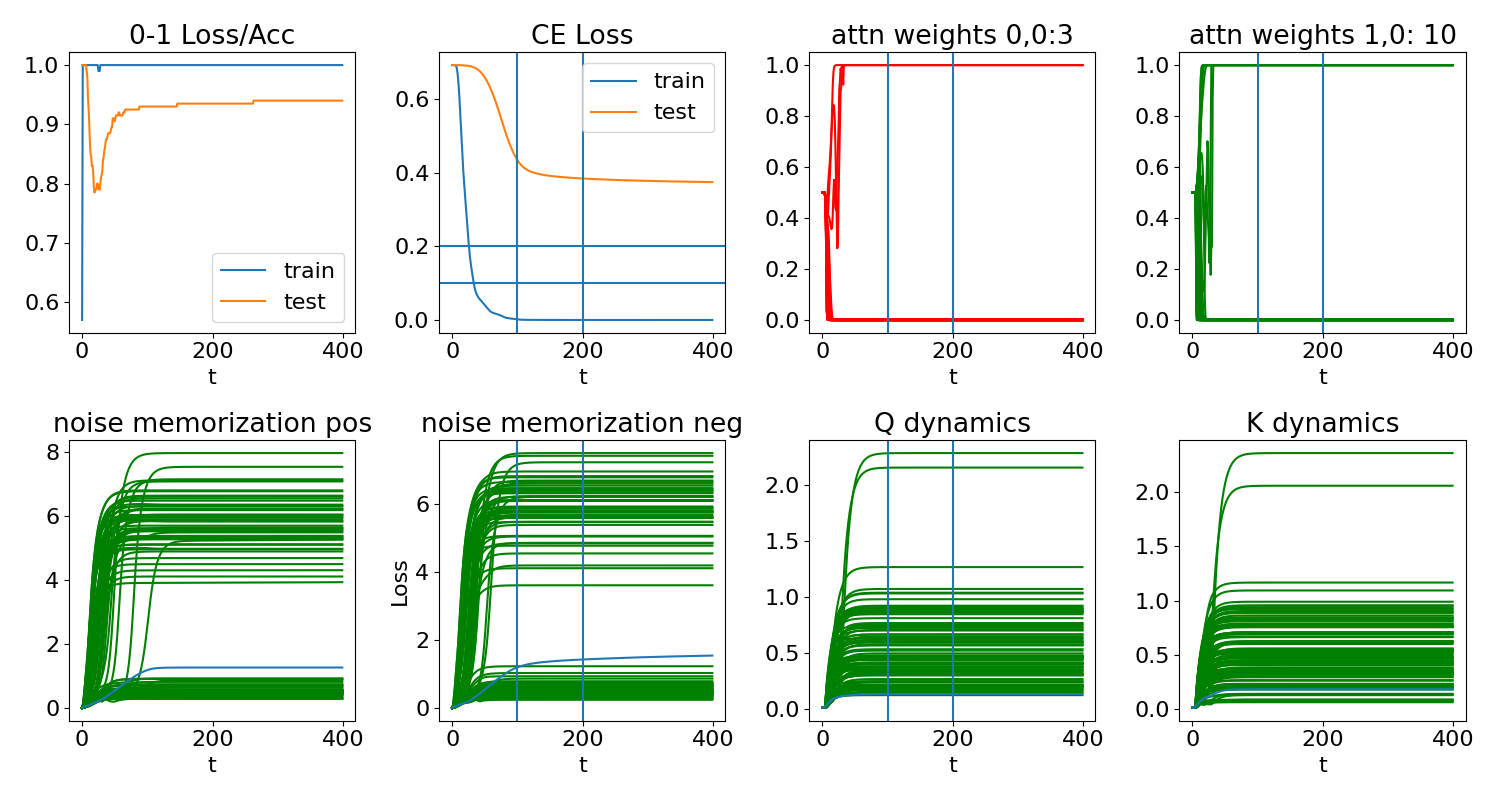}
    \includegraphics[width=0.9\textwidth]{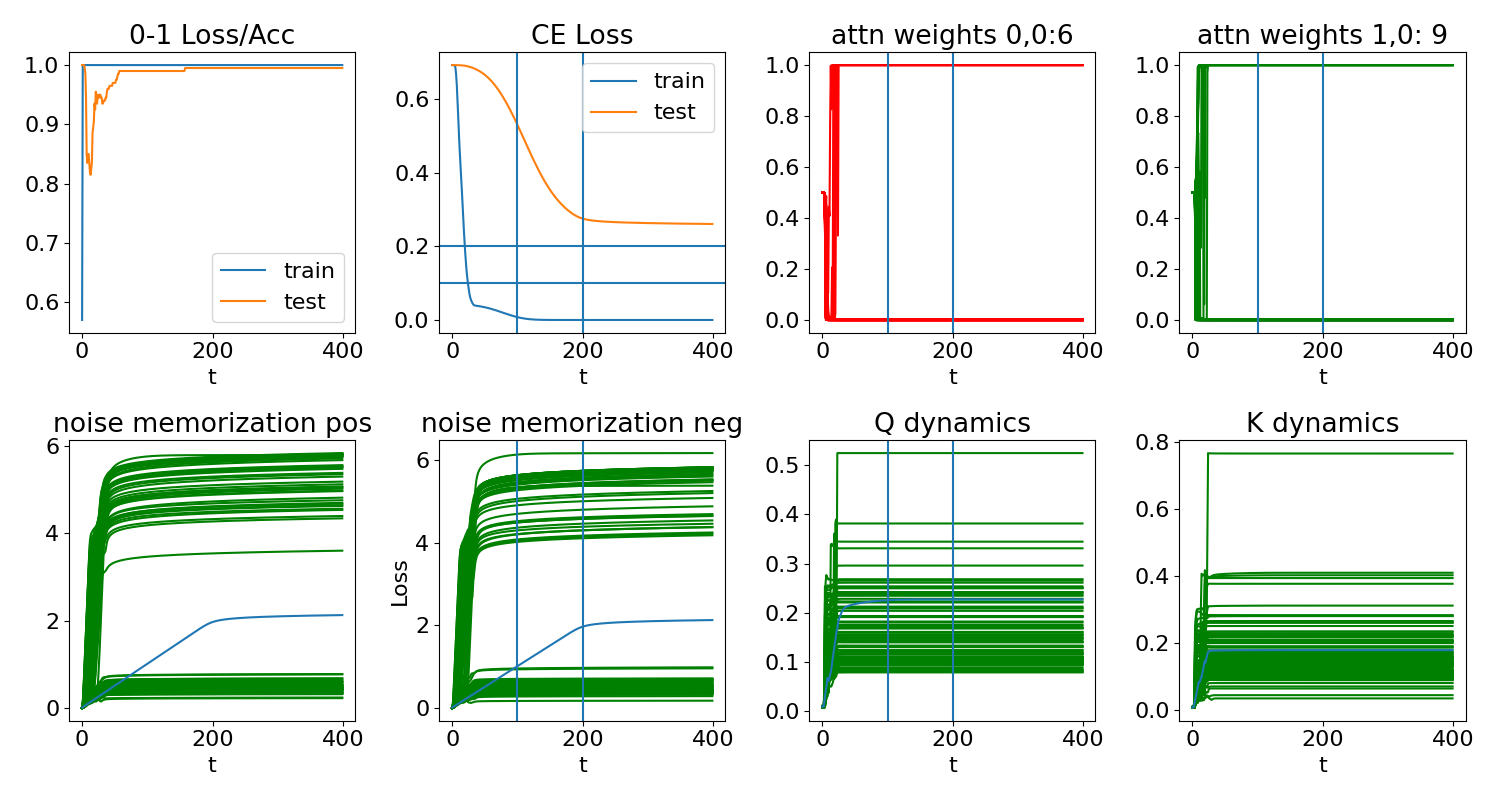}
    \includegraphics[width=0.9\textwidth]{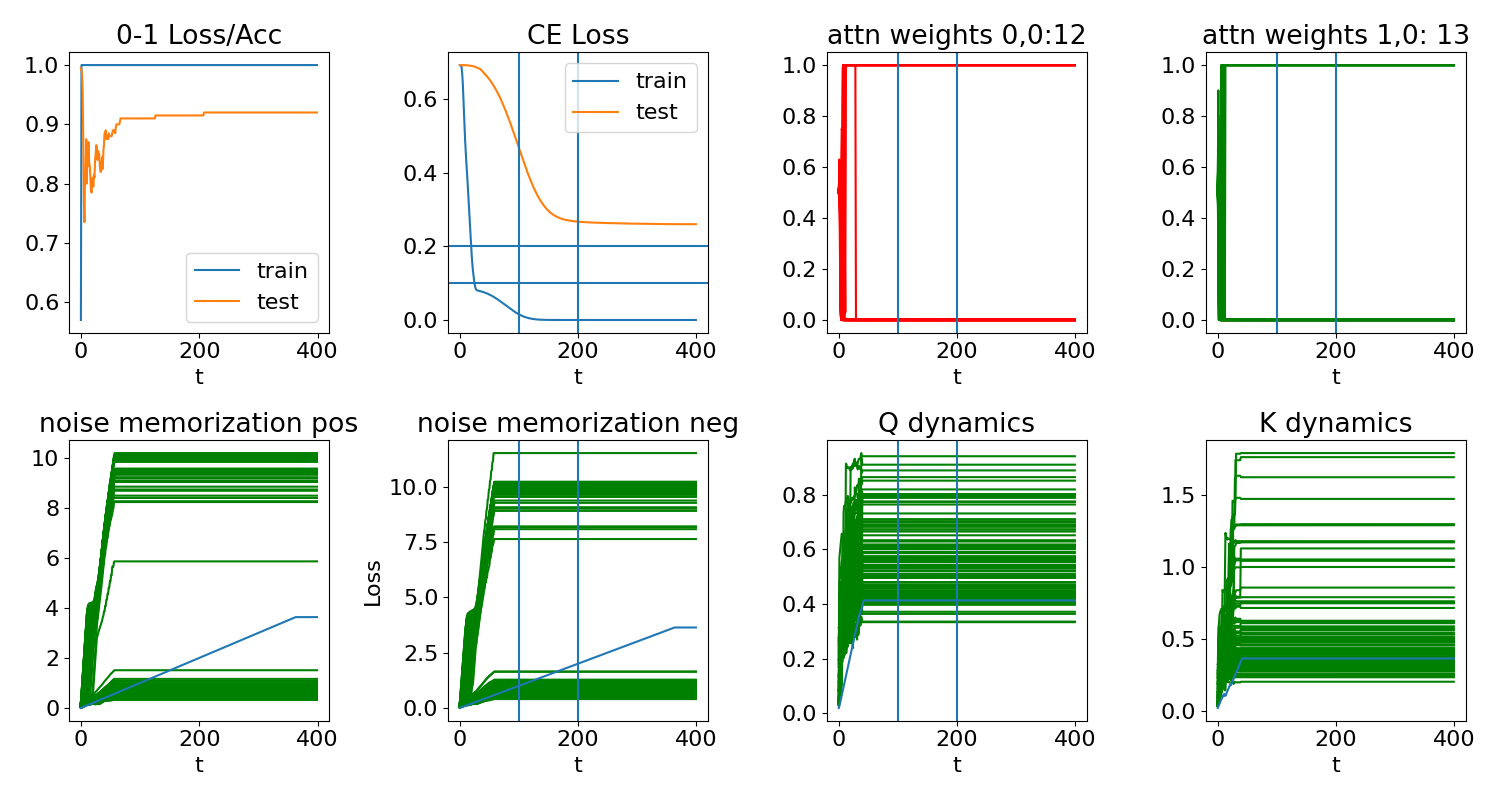}
    \caption{Dynamics, with AttnBinary + ReLU$^3$.
    Line 1: Adam($\eta = 1e-2$). Line 2: signGD1($\eta = 1e-2$). 
    Line 3: signGD2($\eta = 1e-2$).
    }
    \label{fig:dynamics-AttnBinary-ReLU3-1}
\end{figure}

\begin{figure}
    \centering
    \includegraphics[width=0.9\textwidth]{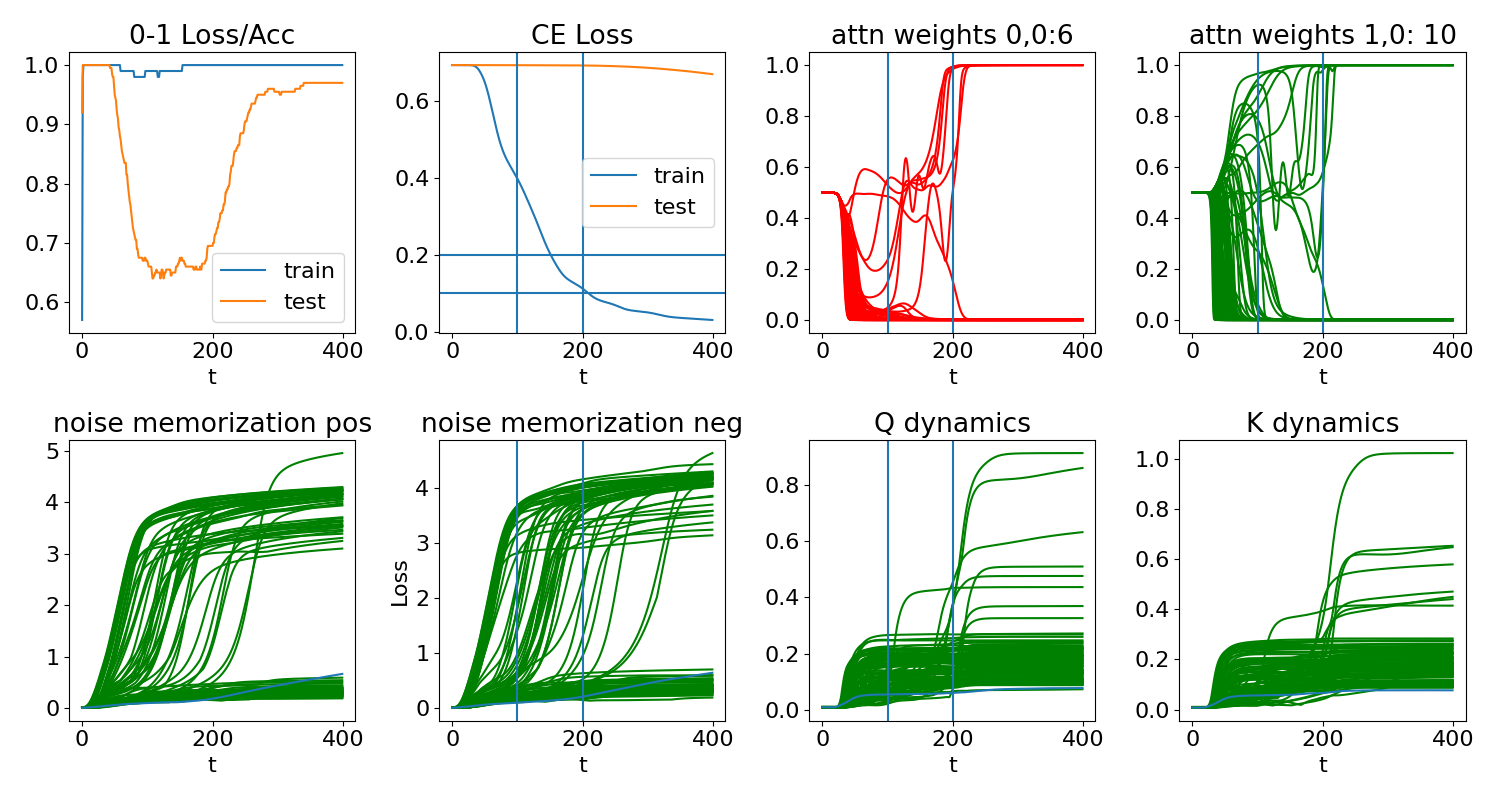}
    \includegraphics[width=0.9\textwidth]{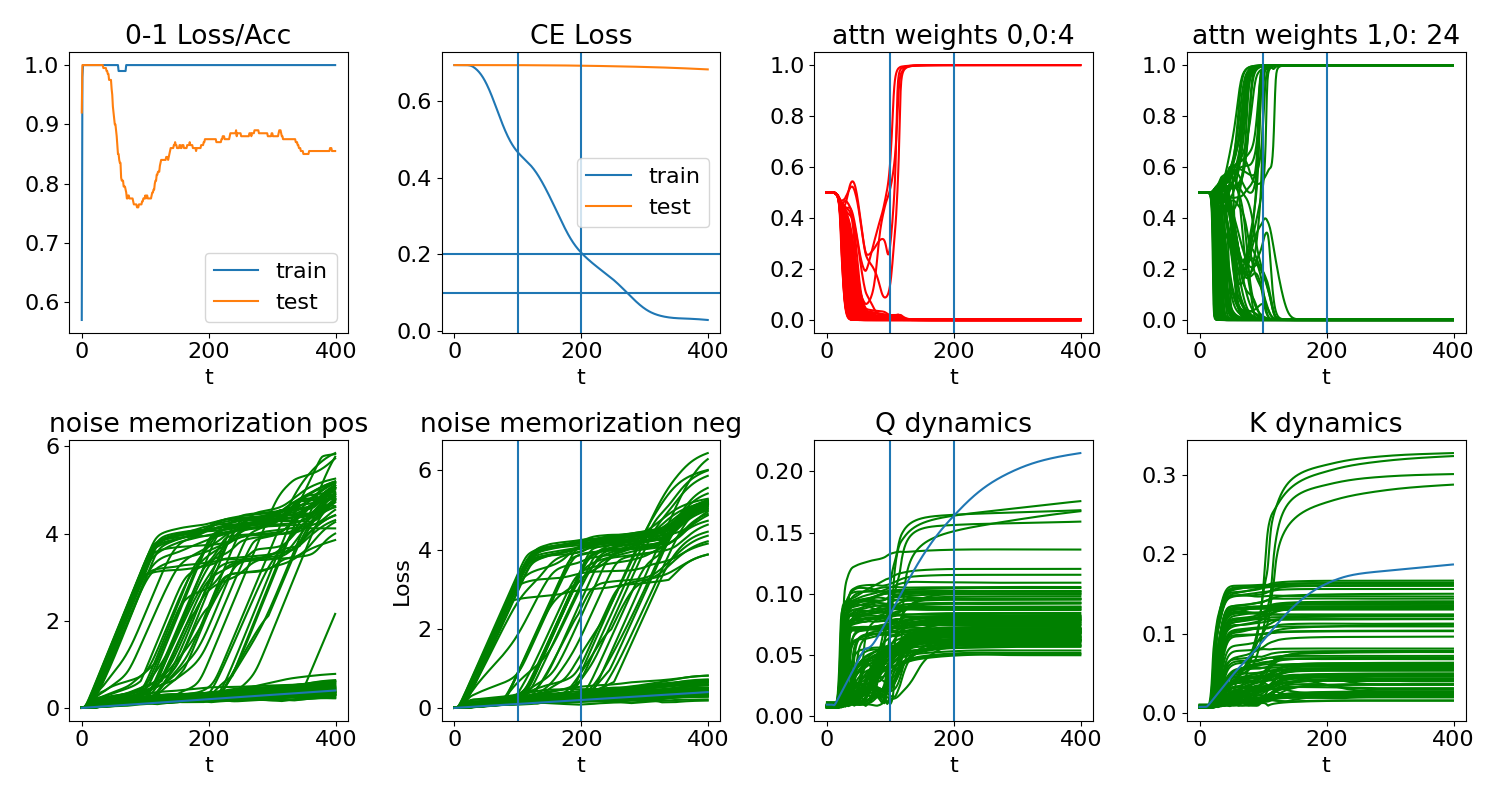}
    \includegraphics[width=0.9\textwidth]{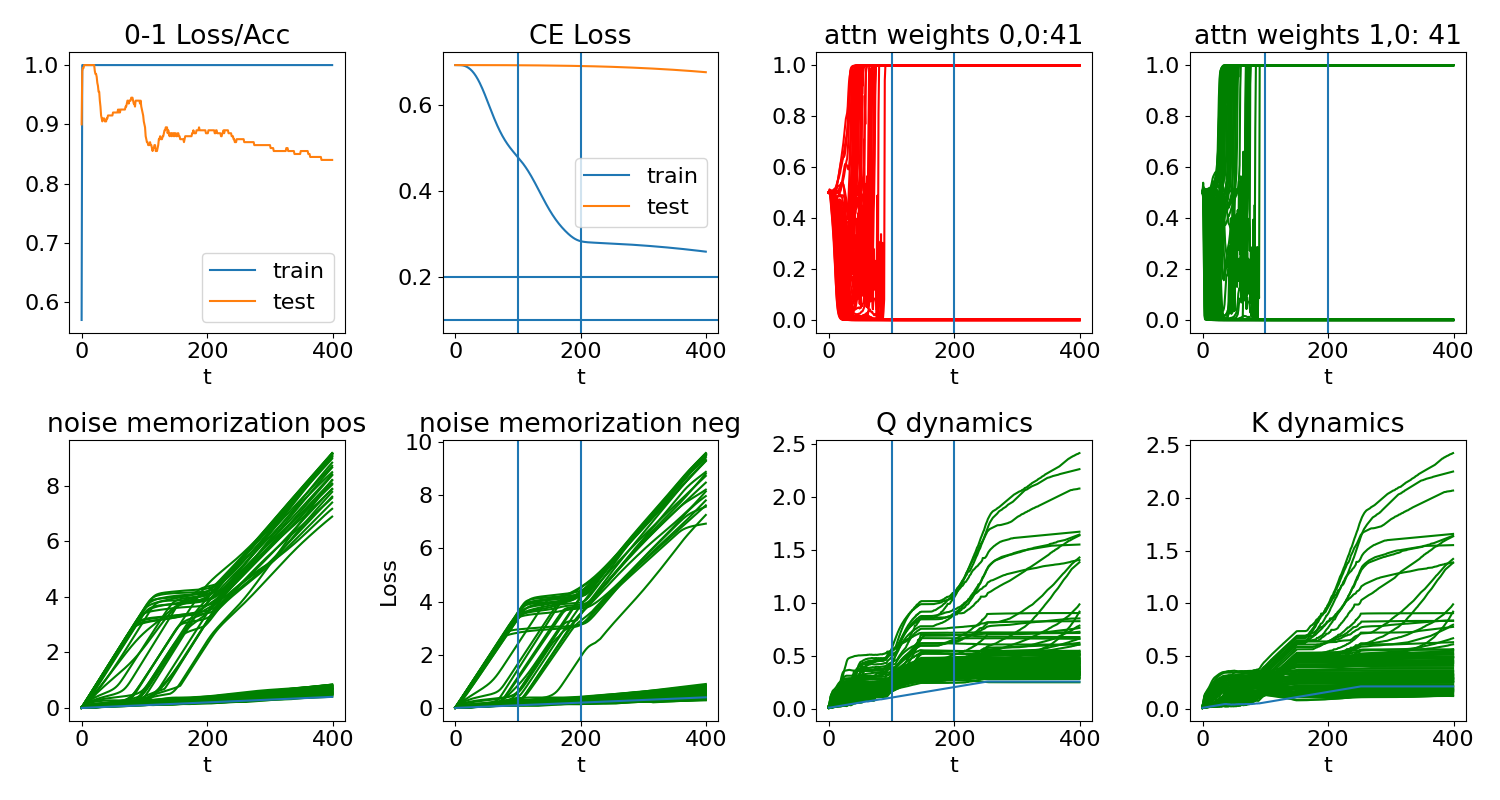}
    \caption{Dynamics, with AttnBinary + ReLU$^3$.
    Line 1: Adam($\eta = 1e-3$). Line 2: signGD1($\eta = 1e-3$). 
    Line 3: signGD2($\eta = 1e-3$).
    }
    \label{fig:dynamics-AttnBinary-ReLU3-2}
\end{figure}

\begin{figure}
    \centering
    \includegraphics[width=0.9\textwidth]{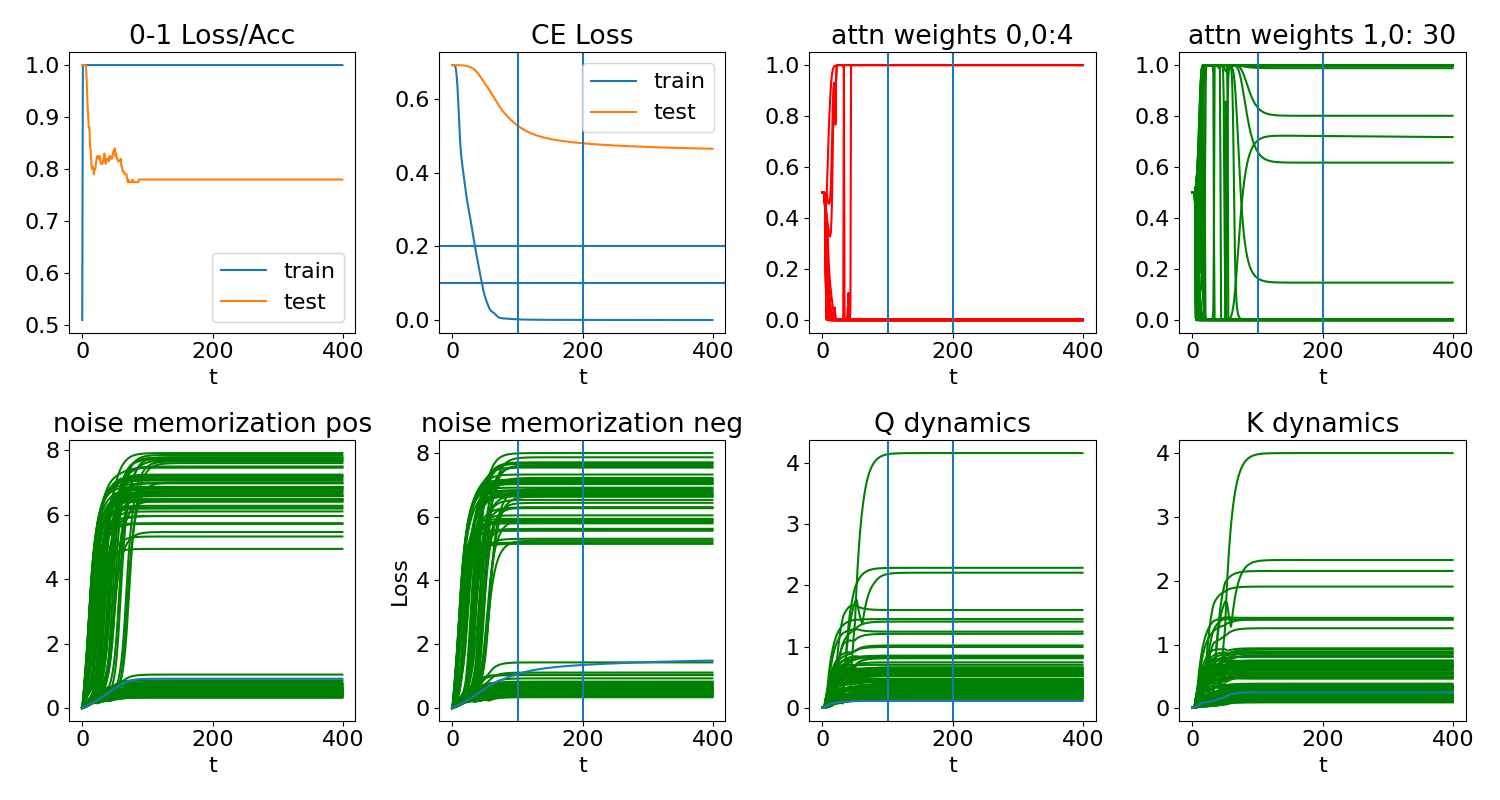}
    \includegraphics[width=0.9\textwidth]{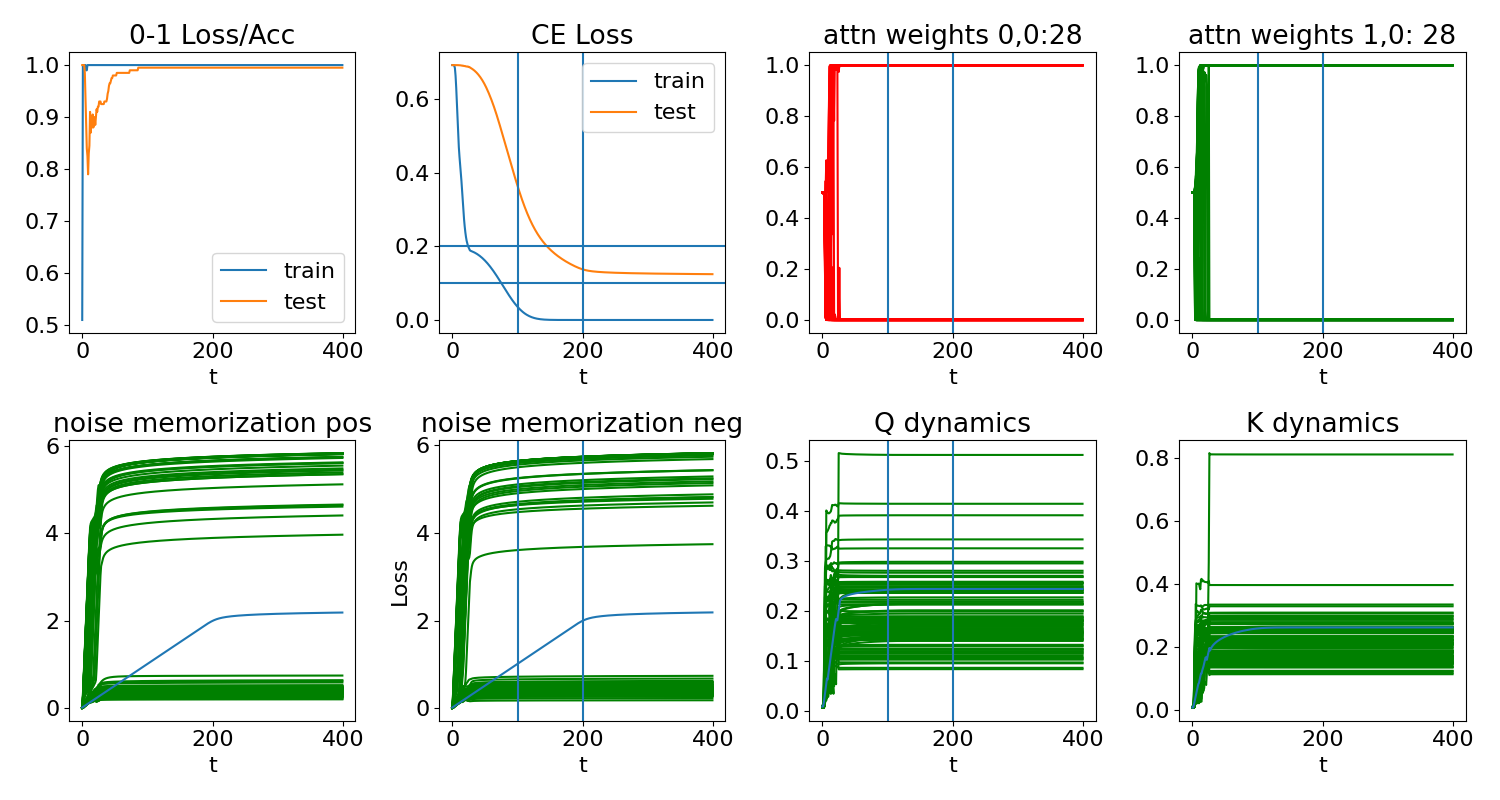}
    \includegraphics[width=0.9\textwidth]{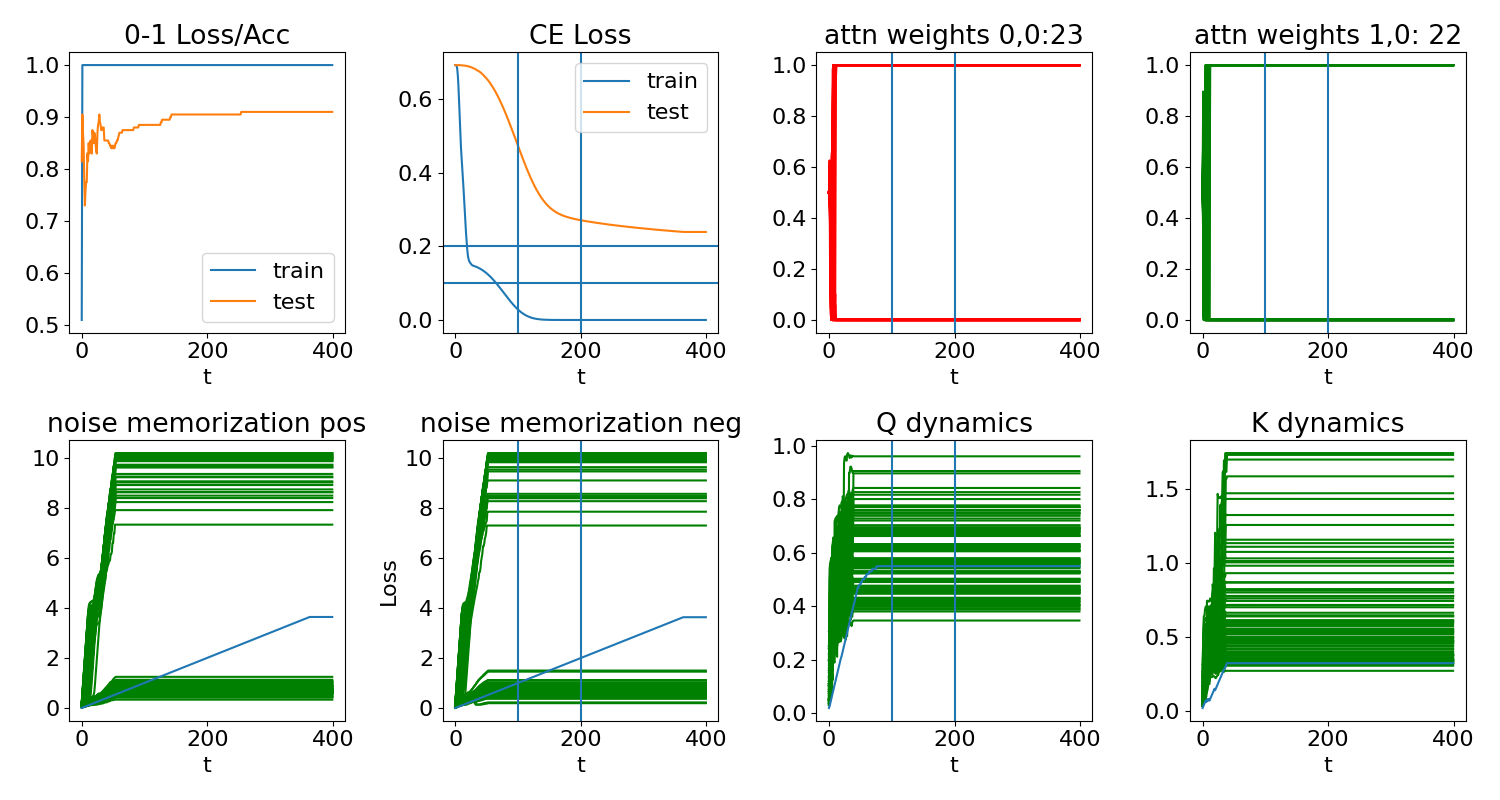}
    \caption{Dynamics, with AttnBinary + ReLU$^3$.
    Line 1: Adam($\eta = 1e-2$). Line 2: signGD1($\eta$=1e-2). 
    Line 3: signGD2($\eta = 1e-2$).
    }
    \label{fig:dynamics-AttnBinaryV-ReLU3-1}
\end{figure}

\begin{figure}
    \centering
    \includegraphics[width=0.9\textwidth]{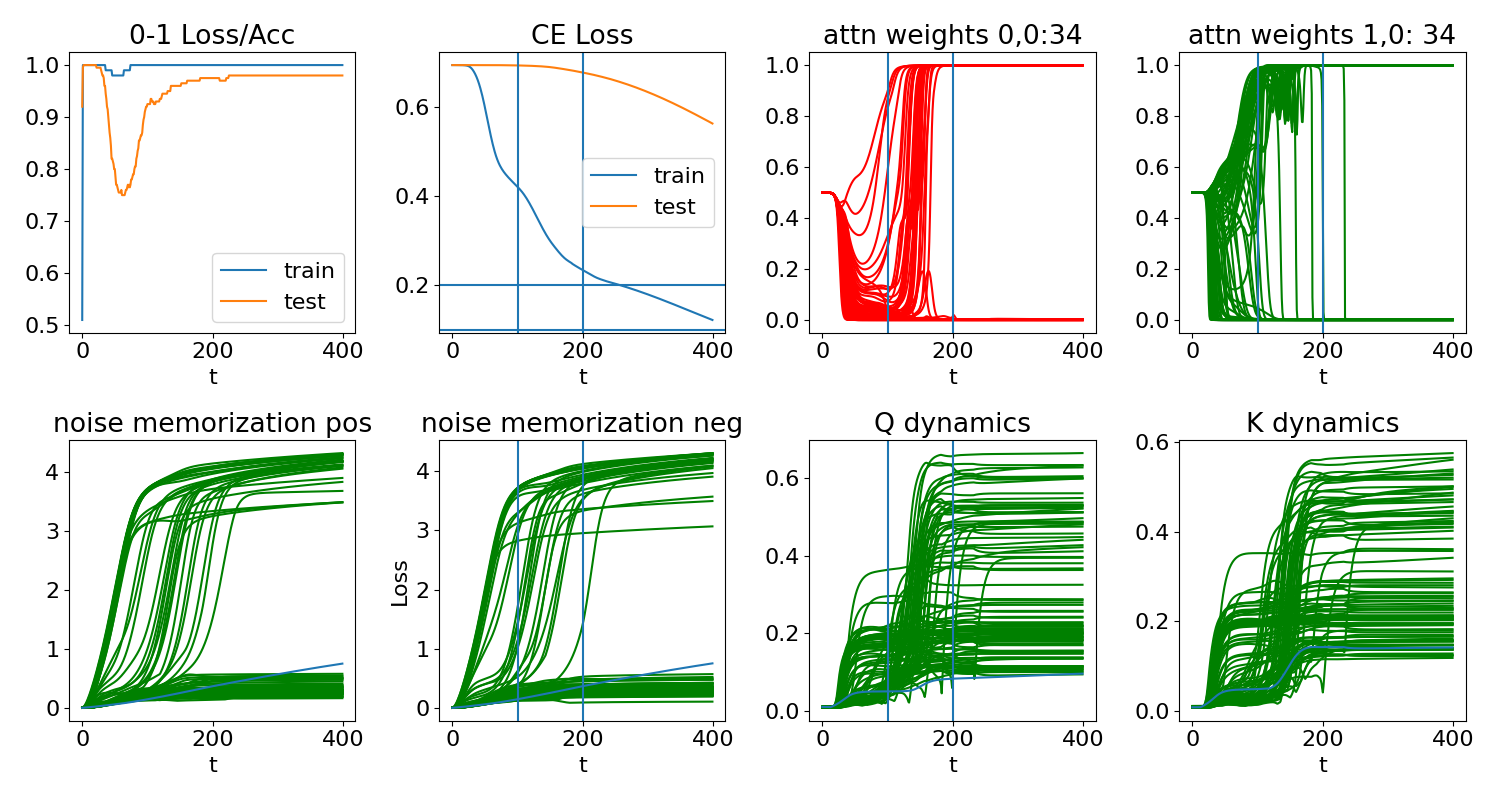}
    \includegraphics[width=0.9\textwidth]{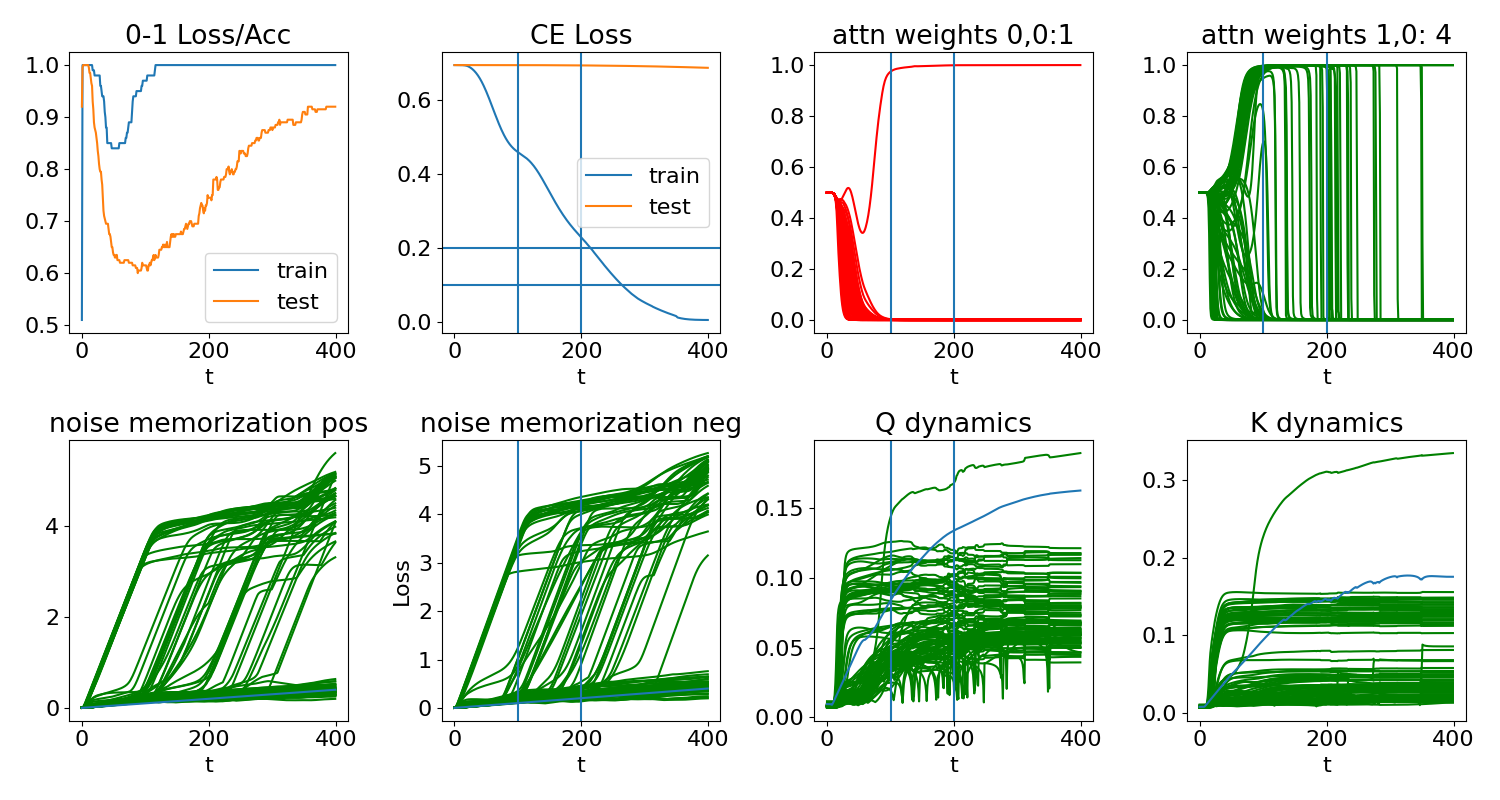}
    \includegraphics[width=0.9\textwidth]{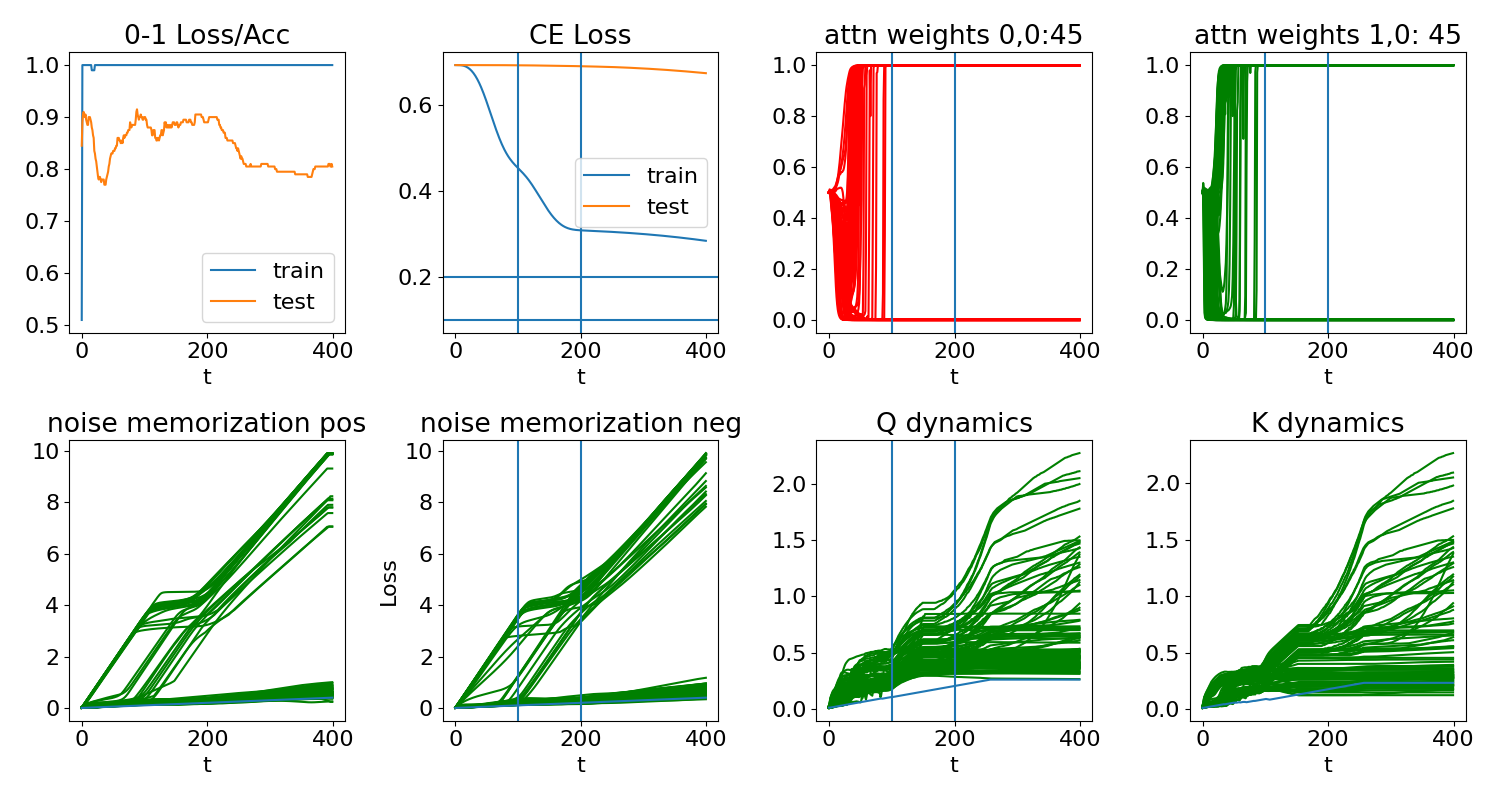}
    \caption{Dynamics, with AttnBinary + ReLU$^3$.
    Line 1: Adam($\eta = 1e-3$). Line 2: signGD1($\eta = 1e-3$). 
    Line 3: signGD2($\eta = 1e-3$).
    }
    \label{fig:dynamics-AttnBinaryV-ReLU3-2}
\end{figure}

\begin{figure}
    \centering
    \includegraphics[width=0.9\textwidth]{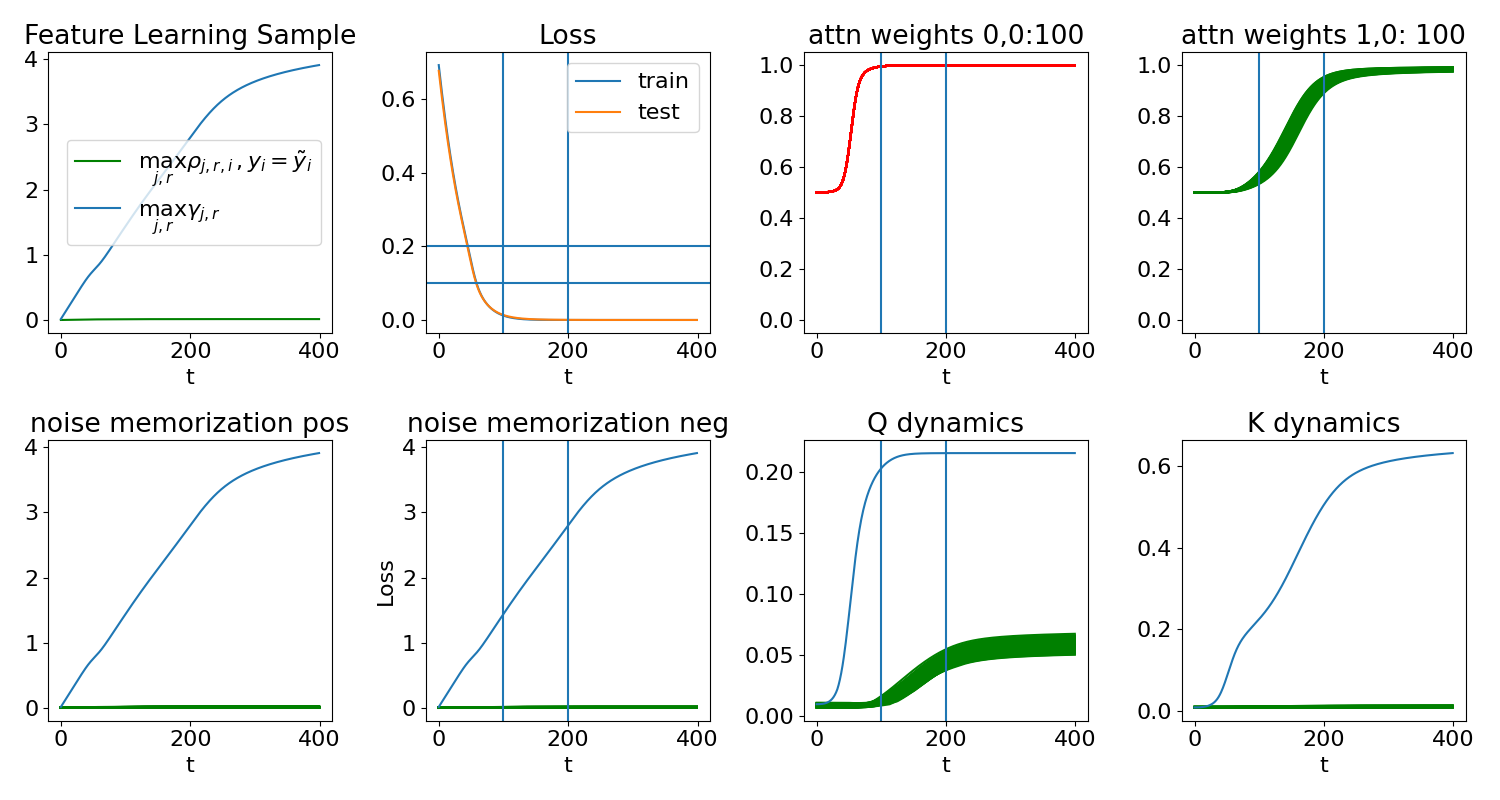}
    \caption{Dynamics, with AttnBinary + linear activation.
    Line 1: normalized GD($\eta = 1e-1$).
    }
    \label{fig:dynamics-normgd}
\end{figure}

\subsubsection{More fine-grained level quantities}
We already know how does feature learning quantities, or say, value inner product evolve in $AttnBinary$ + linear activation model with signGD. Next, we turn to observe the dyanamics of query and key with more fine-grained perspective.
In this section, we care about quantities about attention mechanism listed below, especially for signGD. We aim to answer two questions:
\begin{enumerate}
    \item How does each query and key inner product, i.e., $\langle \wv_{Q,s}, \muv\rangle$, $\langle \wv_{Q,s}, \xiv_i\rangle$,  $\langle \wv_{K,s}, \muv\rangle$, $\langle \wv_{K,s}$, evolve?
    \item How does the change of query and key impact the post-softmax quantities, i.e., attention weightes?
\end{enumerate}
\begin{itemize}
    \item each query and key. Formally, we care about $\langle \wv_{Q,s}, \muv\rangle$, $\langle \wv_{Q,s}, \xiv_i\rangle$,  $\langle \wv_{K,s}, \muv\rangle$, $\langle \wv_{K,s}, \xiv_i\rangle$ for all $i\in[n]$ and $s\in[m_k]$.
\end{itemize}
We use the same hyperparameters as the last section.

\paragraph{Results}
Currently, we have some preliminary results, shown in Fig.~\ref{fig:qksample-signGD2-lr=1e-3},\ref{fig:qkformula-signGD2-lr=1e-3}. 
Fig.~\ref{fig:qksample-signGD2-lr=1e-3} shows the dynamics of query and key inner product: $\langle \wv_{Q,s}, \muv\rangle$, $\langle \wv_{Q,s}, \xiv_i\rangle$,  $\langle \wv_{K,s}, \muv\rangle$, $\langle \wv_{K,s}$. In each plot, the blue line represents the inner product between sampled $\wv_{Q,s}$ or $\wv_{K,s}$ with $\muv$, and the different plots in one line use different sampled neurons (actually we use the first 4 neurons). The green lines represent the inner product of the same query and key parameters with the noise patch in each positive data, while the red lines correspond to negative data. 
Fig.~\ref{fig:qkformula-signGD2-lr=1e-3} shows dynamics of some quantities appeared in the gradient of query and key parameters. Formally, in the left two figures of the first line, we plot $\langle \wv^{(t)}_{K,s}, y_{i}\muv - \xiv_{i}\rangle$ for all $i\in[n]$ and sampled neuron $s$. 
In the left two figures of the second line is $\langle \wv^{(t)}_{Q,s}, s_{i,00}s_{i,01}y_{i}\muv + s_{i,10}s_{i,11} \xiv_{i}\rangle$. 
In the rightest figure of second line, we plot $\langle \bar{\wv}^{(t)}_{V,1} - \bar{\wv}^{(t)}_{V,-1}, y_{i}\muv - \xiv_{i}\rangle$. 
Same as above, green lines represent positive samples, red lines represent negative samples.

Some quick observations are:
\begin{itemize}
    \item $\langle \wv_{Q,s}, \muv \rangle$ and $\langle \wv_{K,s}, \muv \rangle$ go towards opposite direction.
    \item data points with same label have similar trend.
    \item dynamics across different neurons are similar in the sense of symmetry.
    \item removing all the outliers, $\langle \wv_{Q,s}, \xiv_i\rangle$ and $\langle \wv_{K,s}, \xiv_i \rangle$ are similar, going towards same direction with similar magnitude, especially in linear activation. 
    \item architecture with ReLU$^3$ activation has more complicated dynamics.
\end{itemize}

\begin{figure}
    \centering
    \includegraphics[width=0.9\textwidth]{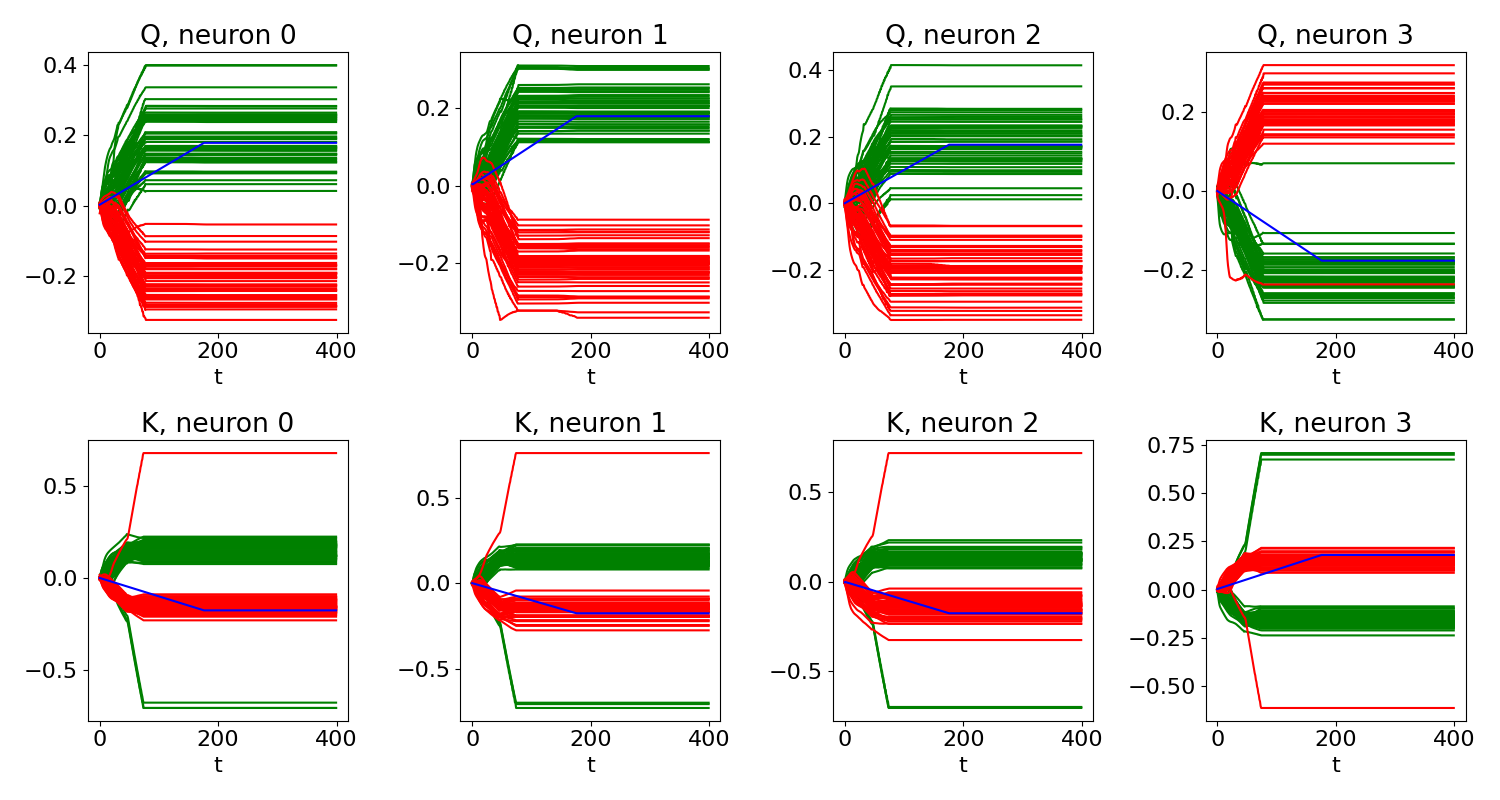}
    \includegraphics[width=0.9\textwidth]{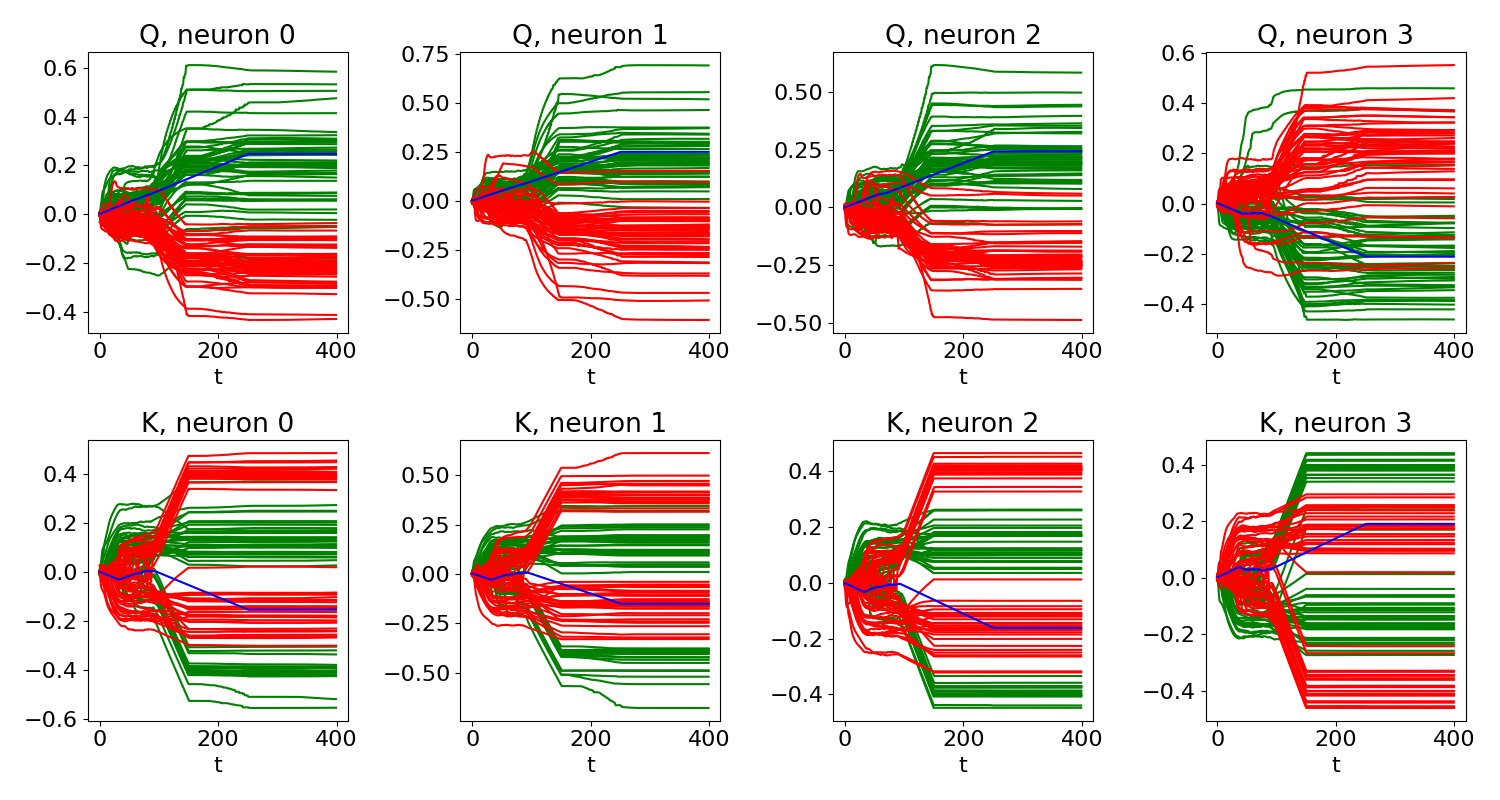}
    \includegraphics[width=0.9\textwidth]{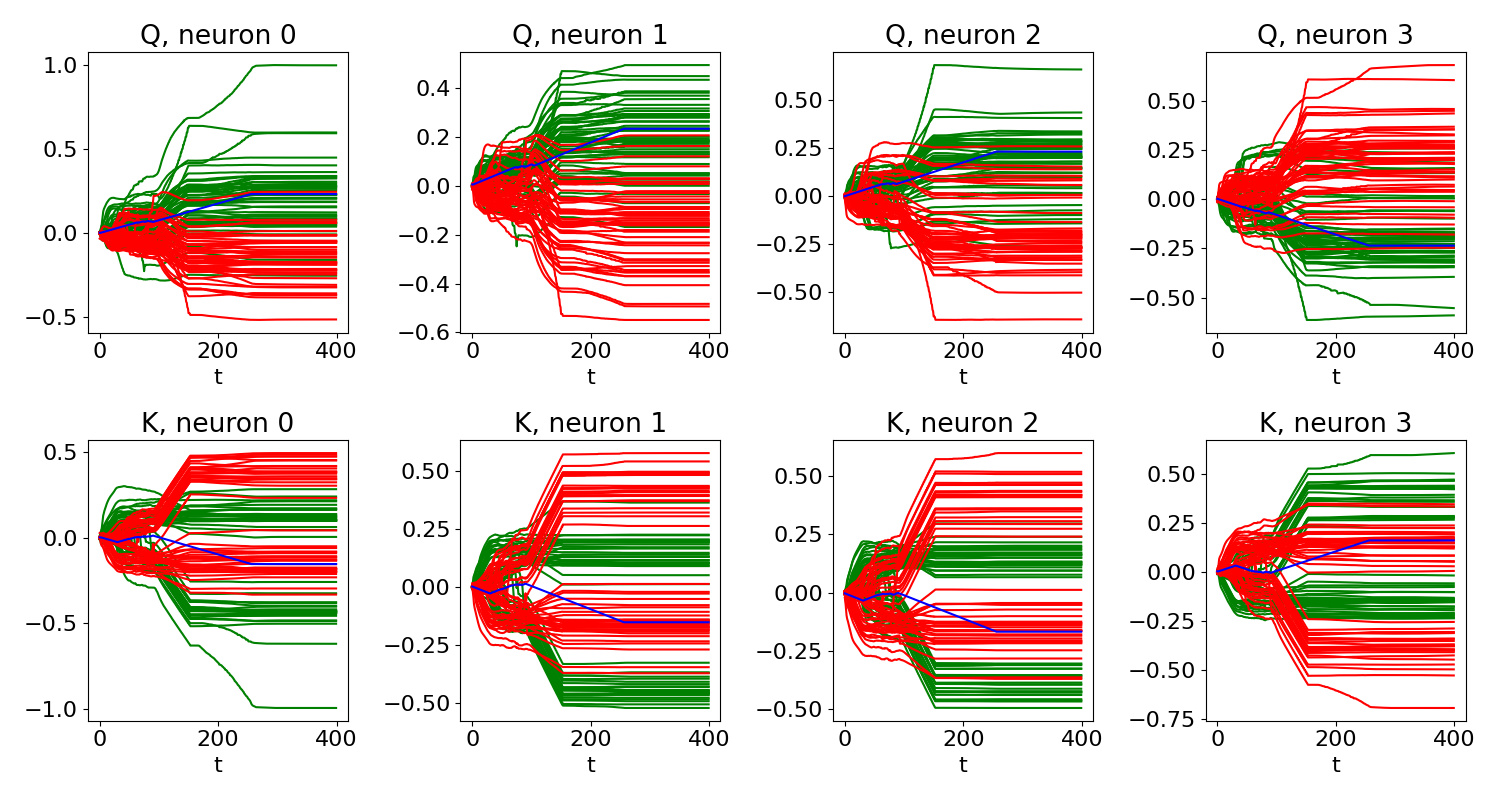}
    \caption{Dynamics of sampled neurons of query and key with all training data input, with signGD2 optimizer and various models. 
    Blue line represents the inner product with (positive) feature patch, while green line is for noise patch in all positive data, red line is for noise patch in all negative data.
    We consistently use learning rate 1e-3.
    Line 1: AttnBinary + linear activation.. Line 2: AttnBinary + ReLU$^3$ activation.
    Line 3: AttnBinaryV + ReLU$^3$ activation.
    }
    \label{fig:qksample-signGD2-lr=1e-3}
\end{figure}

\begin{figure}
    \centering
    \includegraphics[width=0.9\textwidth]{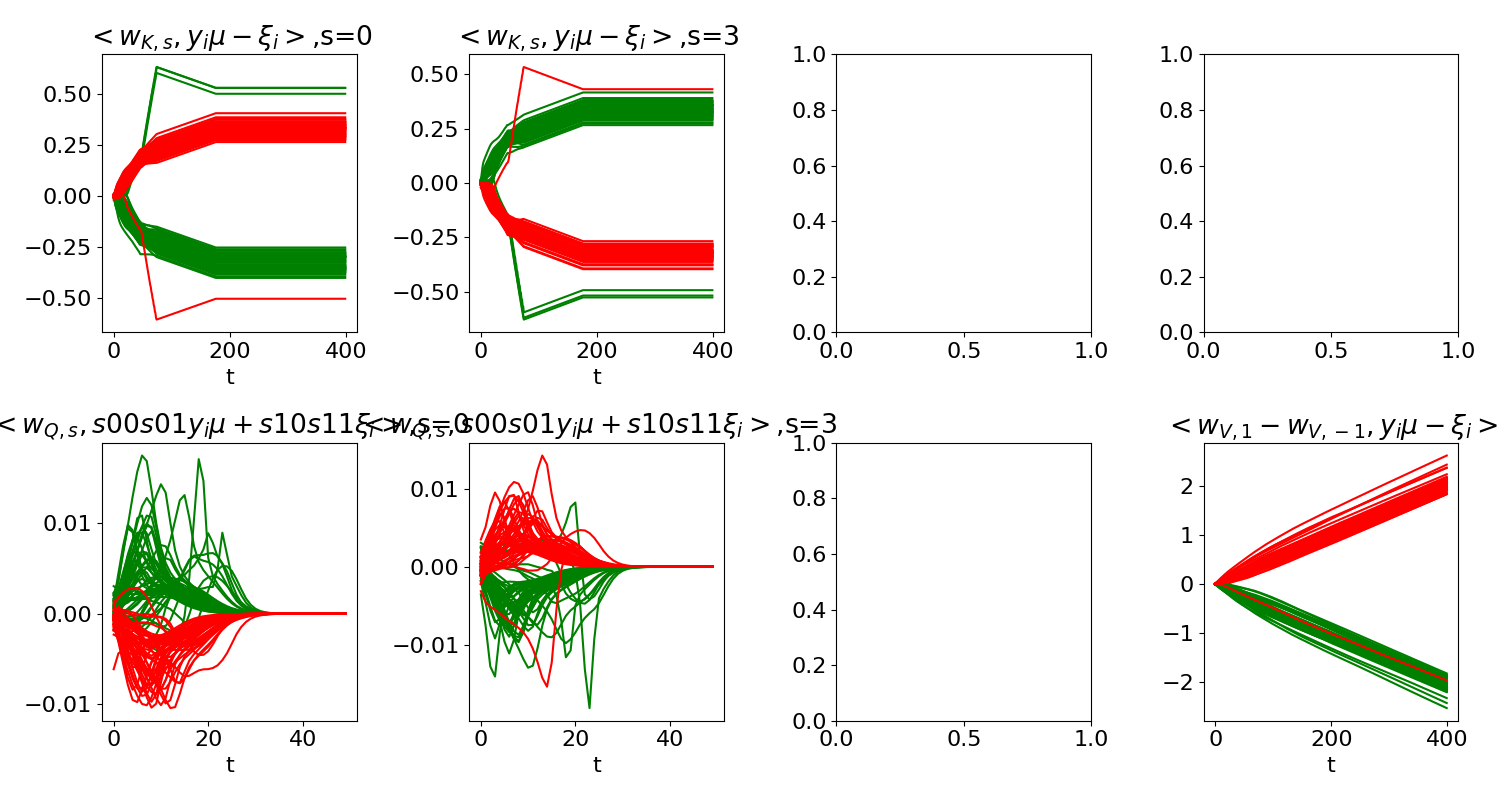}
    \includegraphics[width=0.9\textwidth]{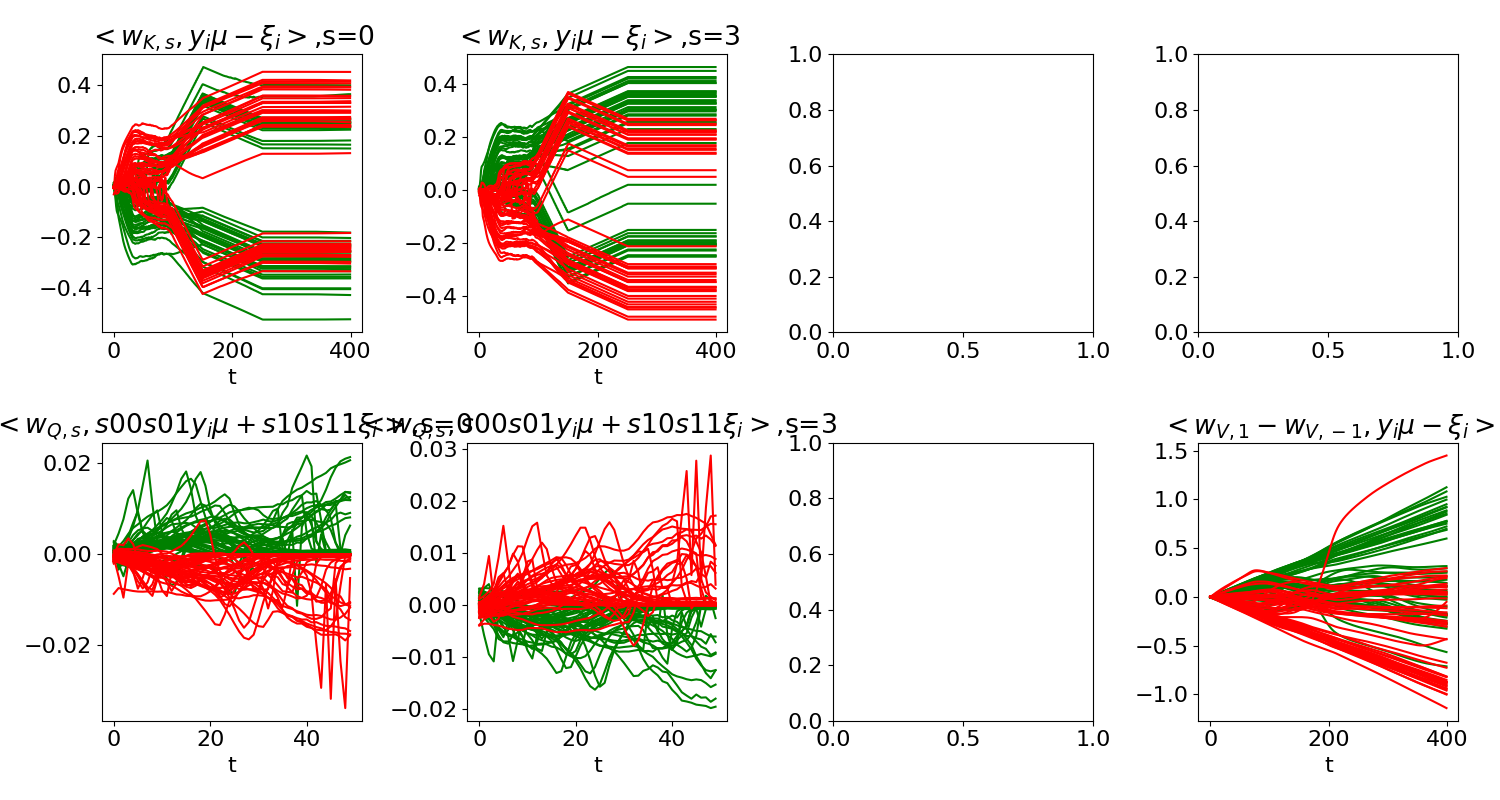}
    \includegraphics[width=0.9\textwidth]{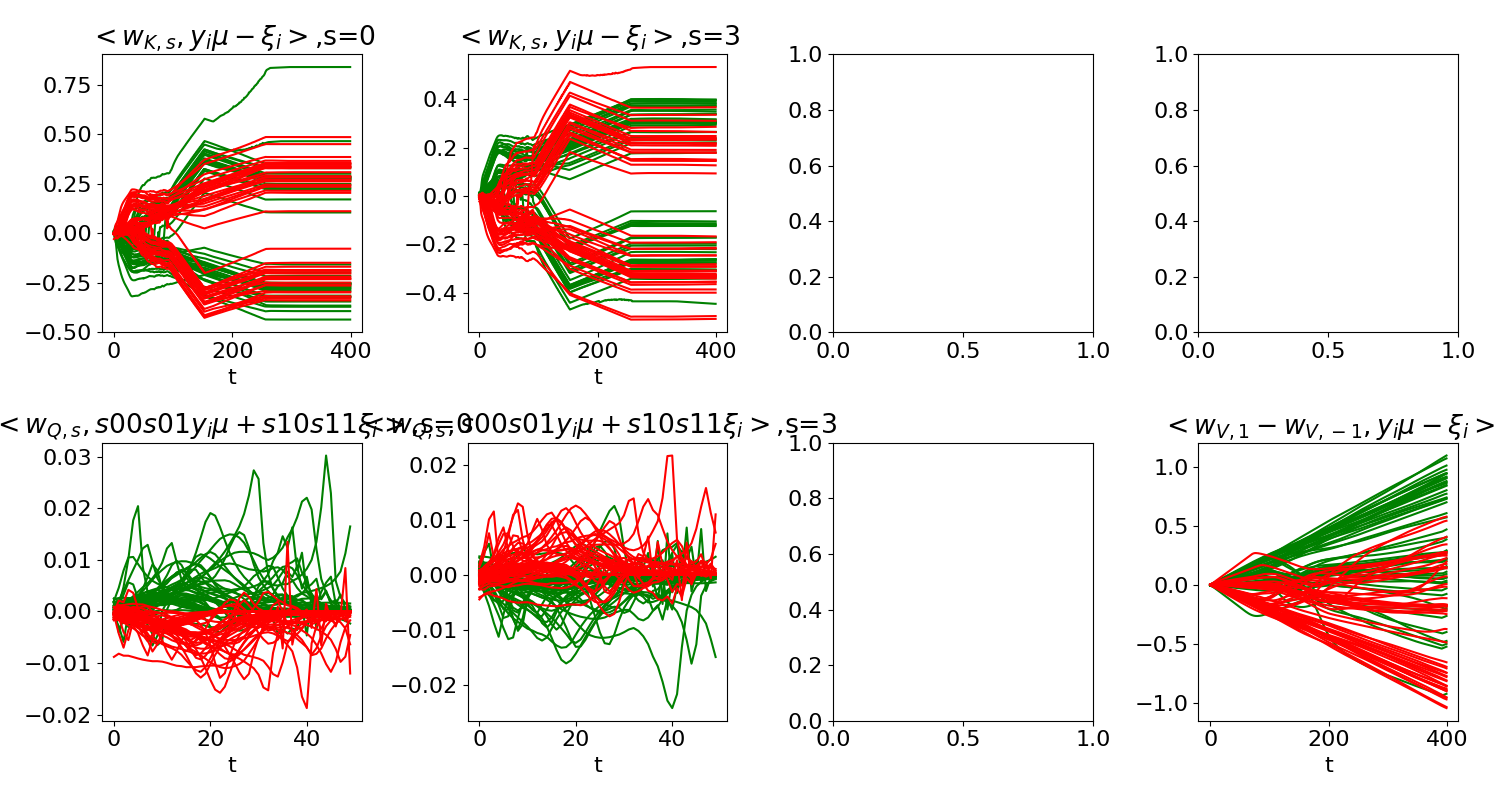}
    \caption{Dynamics of quantities of interest about query and key with all training data input, with signGD2 optimizer and various models. 
    Specifically,  we plot $\langle \wv^{(t)}_{K,s}, y_{i}\muv - \xiv_{i}\rangle$ in upper left, 
    $\langle \wv^{(t)}_{Q,s}, s_{i,00}s_{i,01}y_{i}\muv + s_{i,10}s_{i,11} \xiv_{i}\rangle$ in bottom left for all $i\in[n]$ and sampled neuron $s$,
    and $\langle \bar{\wv}^{(t)}_{V,1} - \bar{\wv}^{(t)}_{V,-1}, y_{i}\muv - \xiv_{i}\rangle$ in bottom right. 
    Green line is for positive data, and red line is for negative data.
    We consistently use learning rate 1e-3.
    Line 1: AttnBinary + linear activation.. Line 2: AttnBinary + ReLU$^3$ activation.
    Line 3: AttnBinaryV + ReLU$^3$ activation.
    }
    \label{fig:qkformula-signGD2-lr=1e-3}
\end{figure}

\subsection{Architectural choices}
\label{sec:arch-choice}
We can make some architectural modifications to make analysis simpler or make settings more realistic. What I have considered include:
\begin{enumerate}
    \item \textbf{Shared attention or not.} Let $\wv_Q$ and $\wv_K$ depend on $j$, which means the attention matrix are separate for positive network and negative network.
    \item \textbf{Position and type of activation function.} Put $\sigma(\cdot)$ on the weighted sum of value, i.e., 
    $\sigma\left(\sum_{a} s_{l,a}\left\langle\wv_{V,j,r}, \xv^{(a)}\right\rangle\right)$. 
    Intuitively, this will lead extra nonlinearity and make analysis more chanllenging.
    But for linear activation, there is no difference.
    \item \textbf{Attention type.} Replace softmax attention with linear attention, i.e., let $s_{l,a} = z_{l,a}$.
    \item \textbf{Scaling on attention.} Here we choose the scaling factor on attention weights as $1$ instead of $\sqrt{m_k}$ in practice. This is because attention weights changes under only $1$-scaling in the range of hyperparameters used.
\end{enumerate}

Now, based on model definition in Section~\ref{sec:notation}, we formally define the modifications we considered above. Recall that the parameters are $\Wv = \left(\Wv_{Q}, \Wv_{K}, \Wv_{V,j} \right)$, where $\Wv_{Q}, \Wv_{K} \in \Rb^{m_k \times d}$ and $\Wv_{V,j} \in \Rb^{m_v \times d}$ for $j \in \set{\pm 1}$. Let $\wv_{V, j, r} = \Wv_{V,j, (\cdot, r)}^{\top}, \wv_{Q, s} = \Wv_{Q, (\cdot, s)}^{\top},  \wv_{K, s} = \Wv_{K, (\cdot, s)}^{\top}$. Then, we have $\wv_{Q, s}, \wv_{K, s}, \wv_{V,j,r} \in \Rb^{d}$. Recall the input $\Xv = \left(\xv^{(1)}, \dots, \xv^{(L)} \right) \in \Rb^{d \times L}$. 

In default, we use shared attention, nonlinearity applied directly to value tensors, softmax attention, and $1$-attention scaling. This is exactly our base model, named by $\mathsf{AttnBinaryV}$, defined as
\begin{align*}
    F_j(\Wv, \Xv) 
    = \frac{1}{m_v}\sum_{l \in [L], r \in [m_v]} \sum_{a=1}^L s_{l,a} \sigma\left(\left\langle\wv_{V,j,r}, \xv^{(a)}\right\rangle\right).
\end{align*}
When the model applies the nonlinearity to the weighted sum value tensors, which is the only difference from $\mathsf{AttnBinaryV}$, we call it $\mathsf{AttnBinary}$. It is defined as
\begin{align*}
    F_j(\Wv, \Xv) 
    = \frac{1}{m_v}\sum_{l \in [L], r \in [m_v]} \sigma\left(\sum_{a=1}^L s_{l,a}\left\langle\wv_{V,j,r}, \xv^{(a)}\right\rangle\right).
\end{align*}

\begin{remark}
    \label{remark:permutation-to-parameter-grad}
    In convolutional model, the position or permutation between patches will not affect the training dynamics, even if the permutation across iterations are different. In current parametrization, this also does not affect the training dynamics. (Thinking the patch index be a intrinsic property instead of permutation, we can see the model output will have no change under different permutations.) But what if we parametrize model with $z_{l,a}$? See discussion in Remark~\ref{sec:comp-spatial}. 
\end{remark}

\subsection{Early writing and experiments}

\subsubsection{Emprical guide for GD analysis}
\begin{enumerate}
    \item (\textbf{High priority}) When attention weights are fixed (particularly for GD), what's the dynamics of $\wv_{V,j,r}$ and the results? Some subquestions are:
    \begin{enumerate}
        \item How to bound $s_{i,j}^{(0)}$ at initialization?
        \item Will $s_{i,j}^{(0)}$, or query $\langle \wv_{Q,s}, \xv\rangle$ \& key $\langle \wv_{K,s}, \xv\rangle$, change (in an unneglectable way)? Can we give a characterization about this? If it is going to change, when will $s_{i,j}^{(0)}$ start to change?
        Given fixed attention type, consider different lr, noise level (i.e., signal-noise ratio and the absolute magnitude of signal and noise). See subsections below for examples.
        \item How to show that training with query \& key parameters (thus attention weights) is indeed better?
    \end{enumerate}
    \item Ideal $N$-stage analysis: 
    \begin{enumerate}
        \item in $[0, T_1]$, only value matrices are updated, attention weights are approximately fixed
        \item in the next stage, attention weights start to change according to the signal-noise ratio. how about value parameters then?
        \item attention weights converge and loss continue to decrease.
    \end{enumerate}
\end{enumerate}

\subsubsection{prior experiments: the learning of attention weights}
Given fixed attention type (here we consider softmax attention), consider different learning rates, noise level (i.e., signal-noise ratio and the absolute magnitude of signal and noise). Will delayed attention weights learning provably happen? When will it happen for a specific setting? 

\subsubsection{$\eta$~is not important}

We first fix feature norm and noise norm (setting feature by 1 and noise level by 0.1), change learning rates to see the results. In summary, \textbf{learning rate $\eta$ only decides the timestep when delayed learning happen and scale everything horizontally.}

When we use GD and $d=m_k=2000,~m_v=20,~\sigma_p=0.1,~\text{mult}=0.1$, which is in the large SNR ratio ($\approx 0.22$), or benign overfitting, regime, the delayed attention weights learning will happen. Within the range of $\eta \in [100, 500]$, the delay threshold is apparent and dependent on $\eta$ ($T \approx 1e4 / \eta$). Roughly, decay attention weights learning happens when loss reaches 0.1.
        
When we use GD and $d=m_k=2000,~m_v=20,~\sigma_p=0.1,~\text{mult}=1.0$, which is in the large SNR ratio thus benign overfitting regime, the delayed attention weights learning will provably happen. And within the range of $\eta \in [0.2, 1]$, the delay threshold is apparent within 400 steps and dependent on $\eta$ ($T \approx 50 / \eta$). Roughly, decay attention weights learning happens when loss reaches 0.2.

\subsubsection{The role of data (absolute) magnitude (by multiplier)}

In this section, we fix feature norm and noise norm (setting feature by 1 and noise level by 0.1), change data magnitude multiplier and see the results. 

Based on above experiments, similarly, when we use GD and $d=m_k=2000,~m_v=20,~\sigma_p=0.1,~\text{mult}=0.5$. The dependence is roughly $T \approx 250 / \eta$ and loss threshold is some value between 0.1 and 0.2 (e.g., 0.15), which implies \textbf{the absolute magnitude will affect the loss value which indicates the happening (or start time) of delayed learning of attention weights. It also affects the learning speed (here by speed we mean the slope in attention weights dynamics) (since we can always pick some learning rate such that the start time is aligned).}

Besides, \textbf{changing data magnitude will not affect whether delayed learning happen.} Set (a)~$\text{mult}=0.1,~\eta=100$, (b)~$\text{mult}=1.0,~\eta=0.5$, (c)~$\text{mult}=5.0,~\eta=0.01 / 0.005$, and fix other hyperparameters as above. 
We see that the dynamics of $s_{1,\cdot}$, or delayed learning starting time ($T=100$), is roughly the same for three runs. 
But for large multiplier, the loss decrease slower and the learning of $s_{0,\cdot}$ are slower and starts earlier. Thus, the delay between learning of values and query \& key become less apparent. 
The point is that increasing multiplier may give different scaling to query \& key, and value matrix, thus decreasing the uniform learning rate is not enough. See Fig.~\ref{fig:multiplier-on-attention-weights}.

\textbf{Finally, we should use small absolute magnitude for both signal and noise to make sure the learning of attention weights is not too early.}

\begin{figure}
    \centering
    \includegraphics[width=1.0\textwidth]{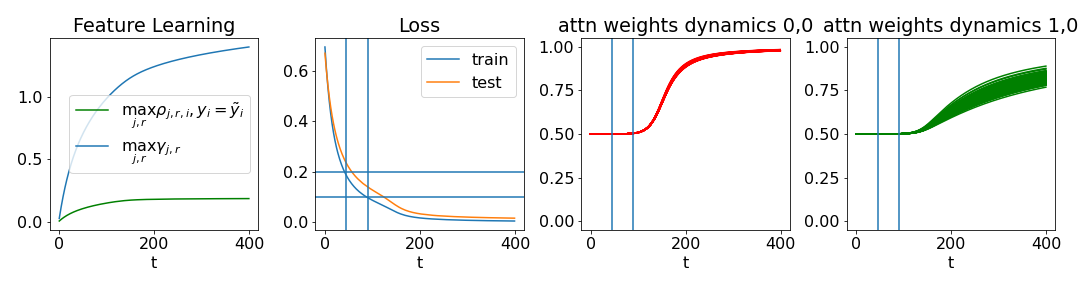}
    \includegraphics[width=1.0\textwidth]{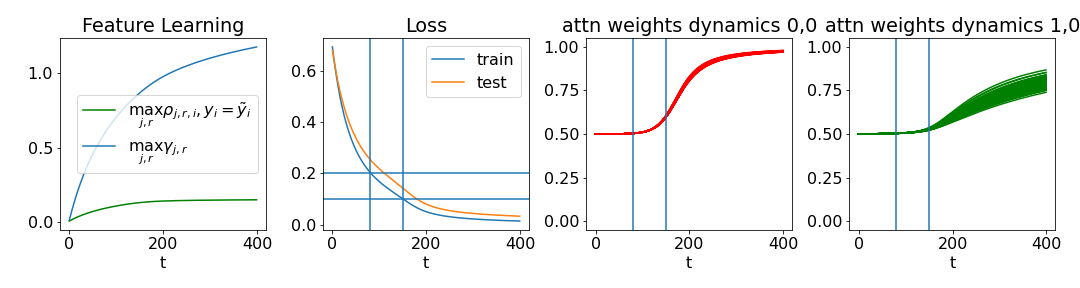}
    \includegraphics[width=1.0\textwidth]{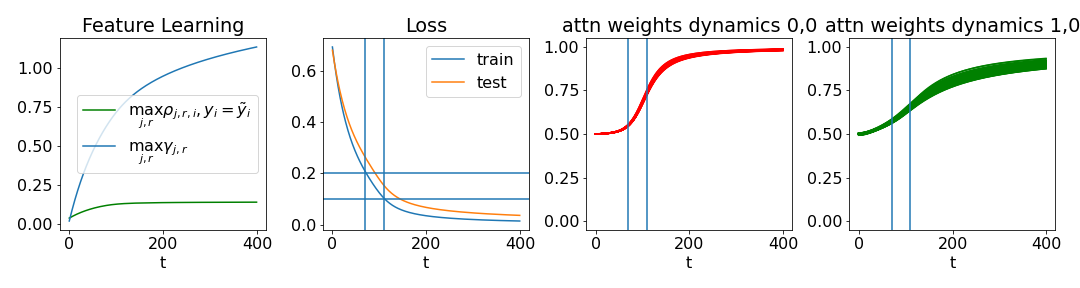}
    \caption{loss and attention weights dynamics under different (data) multiplier and learning rate}
    \label{fig:multiplier-on-attention-weights}
\end{figure}

\subsubsection{The pattern of attention weights learning depends on SNR}

In this section, we fix feature norm (setting feature by 1) and change and noise level. Specifically, we set (a)~$\sigma_p=1/\sqrt{d},~\eta=0.5$, (b)~$\sigma_p=5/\sqrt{d},~\eta=0.5$, (c)~$\sigma_p=8/\sqrt{d},~\eta=2$, (d)~$\sigma_p=12/\sqrt{d},~\eta=5$, and fix other hyperparameters as above. 

Qualitatively, when SNR (noise) is large, the inner product of query \& key w.r.t. noise increase faster compared with inner product w.r.t. feature, thus the $s_{1,\cdot}$ changes faster. And vice versa. In summary, SNR will change the pattern/speed of attention weights learning (here by pattern/speed we mean the difference in $s_{0,0}$ and $s_{1,0}$). 

\begin{figure}
    \centering
    \includegraphics[width=1.0\textwidth]{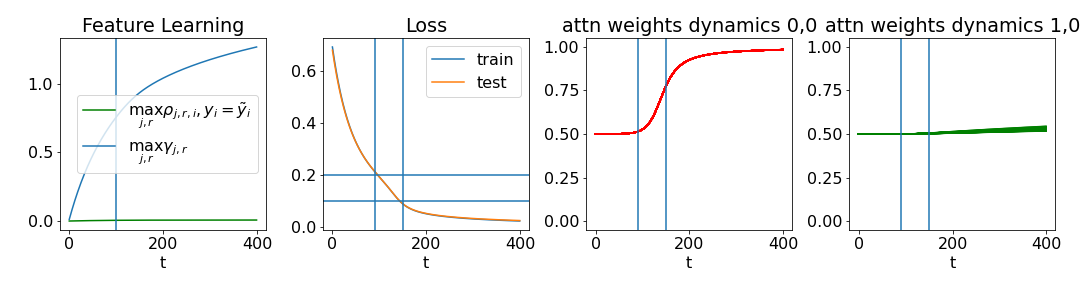}
    \includegraphics[width=1.0\textwidth]{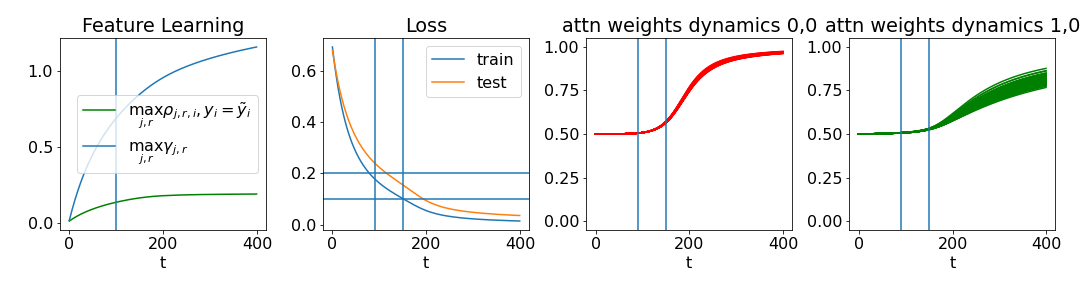}
    \includegraphics[width=1.0\textwidth]{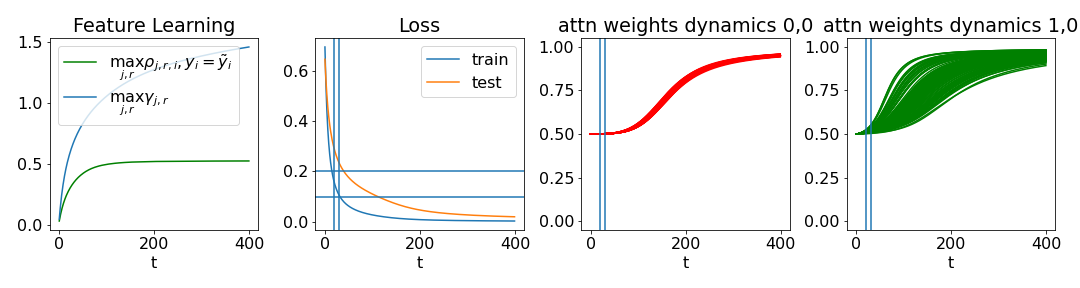}
    \includegraphics[width=1.0\textwidth]{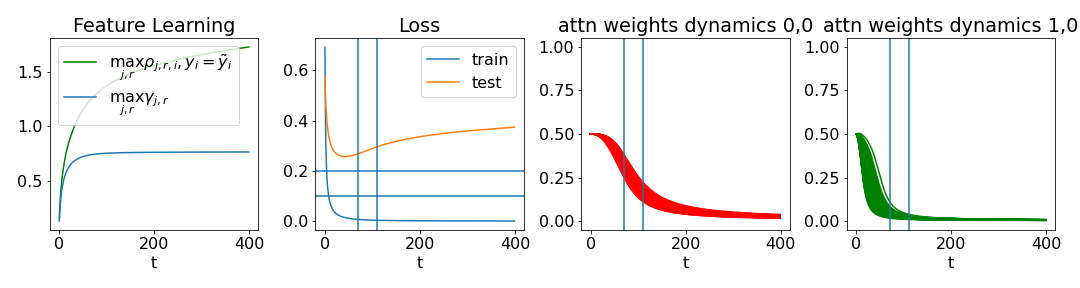}
    \caption{loss and attention weights dynamics under different SNR}
    \label{fig:snr-on-attention-weights}
\end{figure}

\subsubsection{The benefit of self-attention}

The benefit exists but not too surprising. See the Fig~\ref{fig:benefit-of-attention}. The hyperparameters used are $d=m_k=2000,~m_v=20,~\text{mult}=1.0$, and (a) $~\sigma_p = 5 / \sqrt{d},~\eta=0.5$, (b) $~\sigma_p = 12 / \sqrt{d},~\eta=5$.
\begin{figure}
    \centering
    \includegraphics[width=1.0\textwidth]{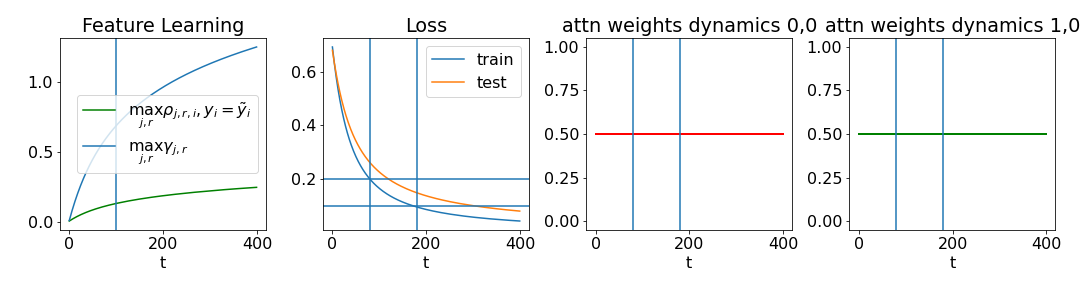}
    \includegraphics[width=1.0\textwidth]{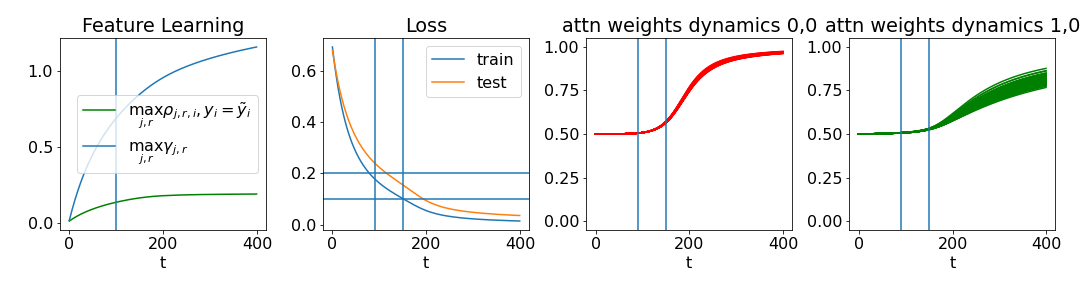}
    \includegraphics[width=1.0\textwidth]{appendix/fig-in-progress/240119-slow-learning-attention-weights/1d_d2000sigma0.2683281572999747mult1.0_tr100_ep400_gd_lr5_aw.png}
    \includegraphics[width=1.0\textwidth]{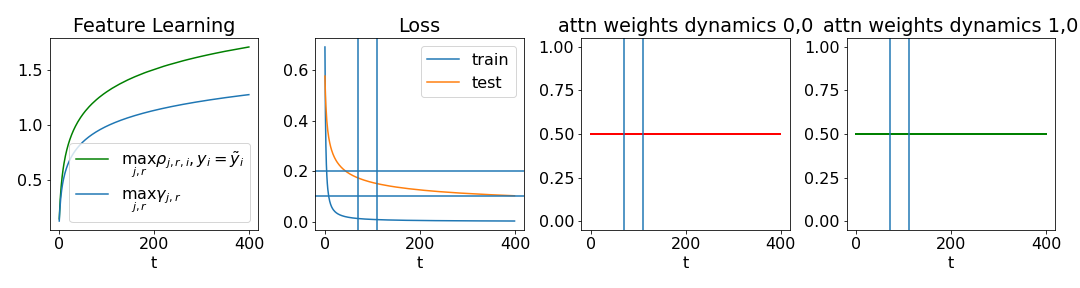}
    \caption{Training with and without query \& key parameters}
    \label{fig:benefit-of-attention}
\end{figure}

\subsubsection{Experiments of Adam}
See Fig.~\ref{fig:benefit-of-attention-adam-feature-learning},\ref{fig:benefit-of-attention-adam-noise-memorization} for learning with and without attention query \& key parameters using Adam optimizer at both feature learning and noise memorization regime. 
Hyperparameters are $d=m_k=2000,~m_v=20,~\text{mult}=1.0$, and (a) $~\sigma_p = 0.2 / \sqrt{d},~\eta=0.01$ in feature learning, (b) $~\sigma_p = 1 / \sqrt{d},~\eta=0.01$ in noise memorization.

\begin{figure}
    \centering
    \includegraphics[width=1.0\textwidth]{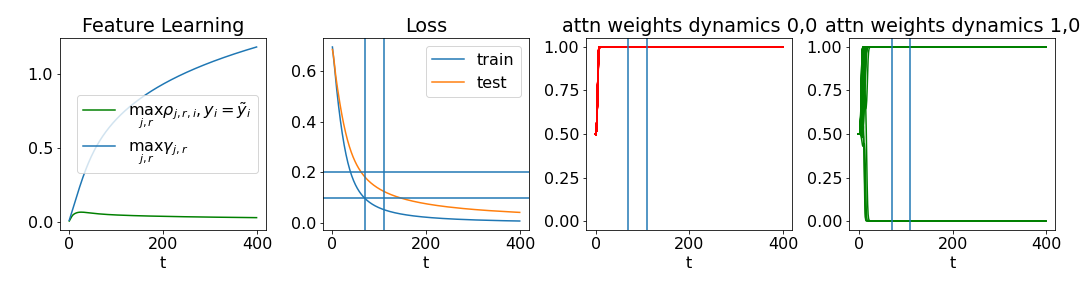}
    \includegraphics[width=1.0\textwidth]{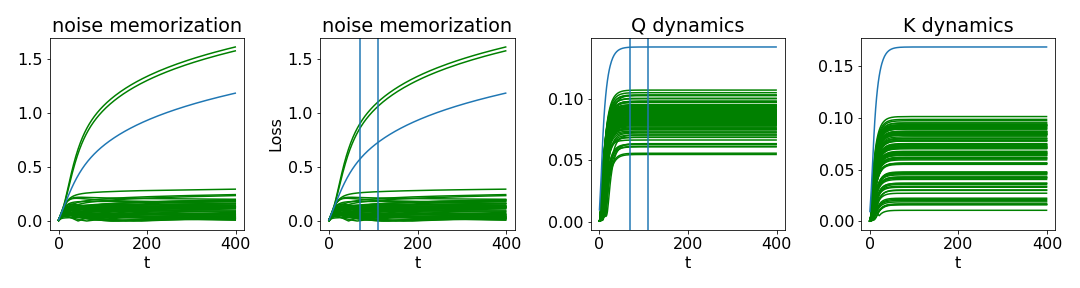}
    \includegraphics[width=1.0\textwidth]{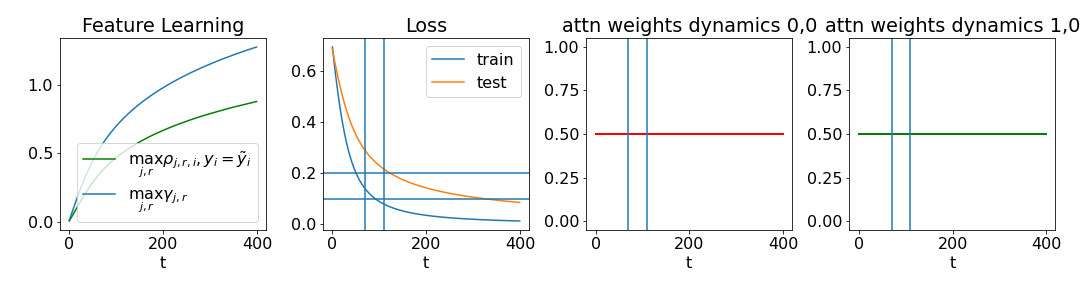}
    \includegraphics[width=1.0\textwidth]{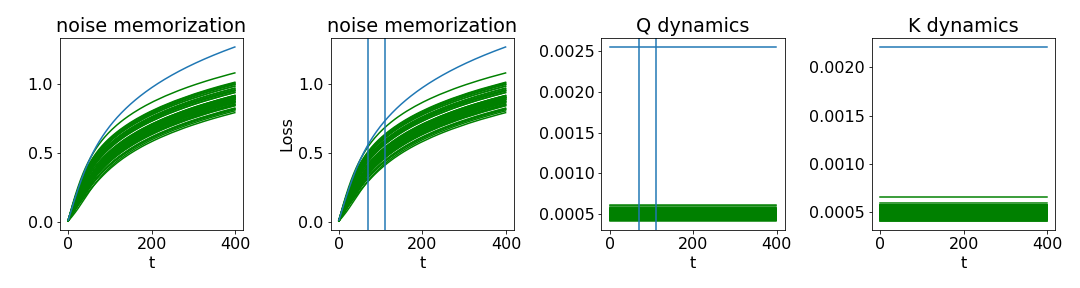}
    \caption{Training with and without query \& key parameters using Adam optimizer. Runs are in feature learning regime}
    \label{fig:benefit-of-attention-adam-feature-learning}
\end{figure}

\begin{figure}
    \centering
    \includegraphics[width=1.0\textwidth]{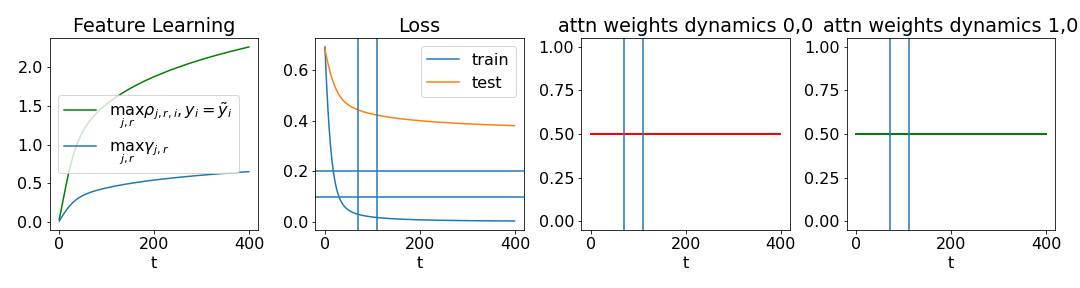}
    \includegraphics[width=1.0\textwidth]{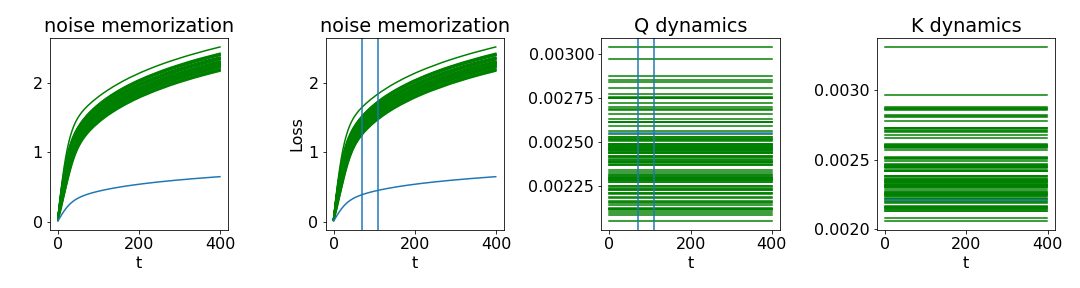}
    \includegraphics[width=1.0\textwidth]{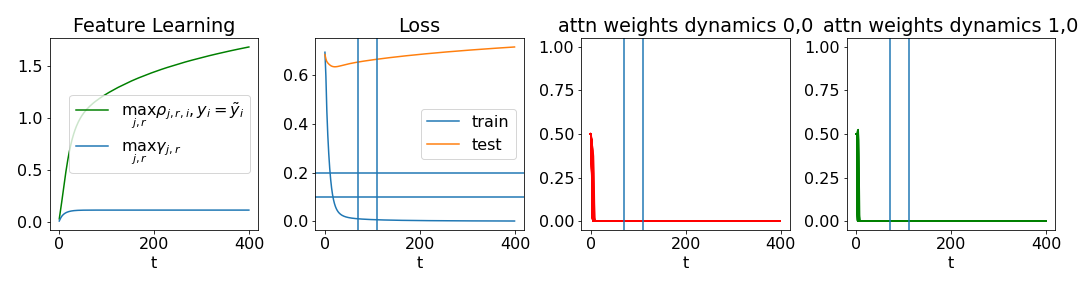}
    \includegraphics[width=1.0\textwidth]{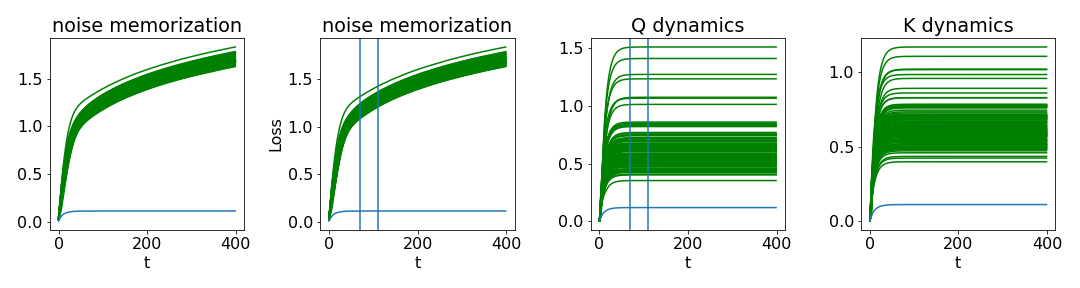}
    \caption{Training with and without query \& key parameters using Adam optimizer. Runs are in noise memorization regime}
    \label{fig:benefit-of-attention-adam-noise-memorization}
\end{figure}
