# Supplementary material for: On the Optimization and Generalization of Two-layer Transformers with Sign Gradient Descent
Source: arXiv:2410.04870 source file (2025-03-02)
Supplement: Supplementary file 6 [file test.tex]

\section{Theoretical Analysis}

The convergence of low-bit optimizers can be guaranteed if their fp32 counterparts converge.
Here we provide a theorem about the convergence of quantized SGDM (Alg.1) under some assumptions. We believe the convergence of low-bit AdamW could be inferred from the convergence of AdamW. 

First, we make some assumptions. The first three are rather standard in stochastic optimization literature, while last two depict properties of  stochastic quantizers. 
\emph{
\begin{myitems}
    \item (Convexity) The objective function is convex and has an unique global minimum $f(\theta^*)$.
    \item (Smoothness) The objective $f(\theta)$ is continuous differentiable and $L$-smooth;
    % i.e. $f(y) - f(x) \le \langle \nabla f(x), y - x \rangle + \frac{L}{2}\norm{x - y}^2$
    \item (Moments of stochastic gradient) The stochastic gradient $g$
    is unbiased, i.e., $\Eb[g(\theta)] = \nabla f(\theta)$, and has bounded variance, i.e.,
    $ \Eb\left[\norm{g(\theta) - \nabla f(\theta)}^2\right] < \sigma^2$, $\forall \theta \in \mathbb{R}^d$.
    \item (Unbiased quantizer)  $\forall x\in \mathbb R^d$, $\Eb\left[Q(x)\right]=x$.
\item (Bounded quantization variance) $\forall x\in \mathbb R^d$, 
$\Eb\left[\norm{Q_m(x)-x}^2\right] \le \sigma_m^2$.
\end{myitems}
}

Then, we have following theorem:
\begin{theorem}
    \label{thm:q-sgdm}
    Consider the Algorithm \ref{alg:framework-sgdm} with Assumptions 1-5. Let $\alpha \in (0, \frac{1-\beta}{L}]$, then for all $T > 0$ we have
    \begin{align}
    \Eb[f(\Bar{{\theta}}_T) - f_*] & \le \frac{1}{2T}\left( \frac{L\beta}{1-\beta} + \frac{1-\beta}{\alpha} \right) \norm{\theta_0 - \theta_*}^2 \nonumber\\
    & + \frac{\alpha \sigma^2}{(1-\beta)}  
    + \frac{\alpha\sigma_m^2}{(1-\beta)}.\label{eqn:convergence-rate}
    \end{align}
    where $\Bar{\theta}_T = \frac{1}{T}\sum_{i=0}^{T-1}\theta_i$.
\end{theorem}

\subsection{Proof of Theorem 1}

To prove Theorem~\ref{thm:q-sgdm}, we need some useful lemmas.

\begin{lemma}
    In Algorithm \ref{alg:framework-sgdm}, The conditional first and second moments of $g_{t}$ satisfies
    \begin{align}
        \Eb[g_{t} | \theta_{t-1}] & = \nabla f(\theta_{t-1}) \\
        \Eb\left[\norm{g_{t}}^2 | \theta_{t-1}\right] & \le \norm{\nabla f(\theta_{t-1})}^2 + \sigma^2
    \end{align}
\end{lemma}

\begin{proof}
    By assumption, we easily have
    \begin{align*}
        \E{g_{t} | \theta_{t-1}} & =
        % \E{Q(\nabla\Tilde f(\theta_{t-1}))} \\ & =
        % \E{\nabla\Tilde f(\theta_{t-1})} \\ & =
        \nabla f(\theta_{t-1}).
    \end{align*}
    % And when $i>1$ we have
    % \begin{align*}
    %     \E{g_{t, i} | \theta_{t-1}} & =
    %     \E{Q(g_{t, i-1} + \nabla\Tilde f(\theta_{t-1})) | \theta_{t-1}} \\ & = 
    %     \E{(g_{t, i-1} + \nabla\Tilde f(\theta_{t-1})) | \theta_{t-1}} \\ & = 
    %     \E{g_{t, i-1} | \theta_{t-1}} + \E{\nabla\Tilde f(\theta_{t-1})} \\ & = 
    %     \E{g_{t, i-1} | \theta_{t-1}} + \nabla f(\theta_{t-1})
    % \end{align*}
    % By reduction it gives the first part of Lemma 1
    % \begin{align*}
    %     \E{g_{t, i} | \theta_{t-1}} = i\nabla f(\theta_{t-1})
    % \end{align*}
    With Assumption 3, it holds true that
    \begin{align*}
        \E{\norm{g(\theta)}^2} &= \E{\norm{g(\theta) - \nabla{f}(\theta) + \nabla{f}(\theta)}^2} \\ &=
        \E{\norm{g(\theta) - \nabla{f}(\theta)}^2} + \E{\norm{\nabla{f}(\theta)}^2} + 2\E{\left\langle g(\theta) - \nabla{f}(\theta), \nabla{f}(\theta) \right\rangle} \\ &=
        \E{\norm{g(\theta) - \nabla{f}(\theta)}^2} + \E{\norm{\nabla{f}(\theta)}^2} \\ &\le
        \sigma^2 + \norm{\nabla{f}(\theta)}^2,
    \end{align*}
    which implies the second part.
\end{proof}

\begin{lemma}
If Assumptions 3-5 hold, then sequence $\{z_t\}$ satisfies
    %Let $\delta_p$, $\delta_g$ and $\delta_m$ be the minimal quantization interval of parameters gradient, and momentum respectively.
    %The 
    \begin{align}
        % z_{t+1} - z_{t} & = \frac{1}{1 - \beta} (\theta_{t+1} - \theta_t) - \frac{\beta}{1 - \beta}(\theta_t - \theta_{t-1}) \\
        % \Eb[z_{t+1} - z_{t}] & = \frac{-\alpha}{1 - \beta} \nabla f(\theta_t) \\
        % \Eb[\norm{z_{t+1} - z_{t}}^2] 
        % & \le  \left(\frac{\alpha}{1-\beta}\right)^2 \left( \Eb[\norm{\nabla f(\theta_t)}^2] + \sigma^2 + \sigma_m^2 \right) + \frac{1 + \beta^2}{(1 - \beta)^2} \sigma_p^2.
        z_{t+1} - z_{t} & = \frac{1}{1 - \beta} (\theta_{t+1} - \theta_t) - \frac{\beta}{1 - \beta}(\theta_t - \theta_{t-1}) \\
        \Eb[z_{t+1} - z_{t}] & = \frac{-\alpha}{1 - \beta} \nabla f(\theta_t) \\
        \Eb[\norm{z_{t+1} - z_{t}}^2] 
        & \le  2\left(\frac{\alpha}{1-\beta}\right)^2 \left(\Eb[\norm{g_{t+1}}^2] + \sigma_m^2  \right).
    \end{align}
\end{lemma}

\begin{proof}
    By definition of $z_t$, we have the first equation immediately.
    Take expectation on the first equation and we get
    \begin{align*}
        \E{z_{t+1}-z_t} &= \frac{1}{1-\beta}\E{\theta_{t+1}-\theta_{t}} - \frac{\beta}{1-\beta}\E{\theta_{t}-\theta_{t-1}}.
    \end{align*}
    Note that
    \begin{align*}
        \E{\theta_{t+1}-\theta_{t}} &= \E{\theta_{t+1} - (\theta_{t} - \alpha m_{t+1})} - \E{\alpha m_{t+1}} \\ &=
        -\alpha\E{m_{t+1}} \\ &=
        -\alpha\E{\beta m_{t} + g_{t+1}} \\ &=
        -\alpha\beta\E{m_{t}} - \alpha \nabla f(\theta_{t}),
    \end{align*}
    and
    \begin{align*}
        \E{\theta_{t}-\theta_{t-1}} &= \E{\theta_{t} - (\theta_{t-1} - \alpha m_{t})} - \E{\alpha m_{t}} \\ &=
        -\alpha\E{m_{t}},
    \end{align*}
    which gives the second equation.
    \begin{align*}
        % \E{z_{t+1}-z_t} &= -\frac{\alpha\beta}{1-\beta}\E{m_{t}} - \frac{\alpha N}{1-\beta}\nabla f(\theta_{t}) + \frac{\alpha\beta}{1-\beta}\E{m_t} \\ &=
        % \frac{-\alpha N}{1-\beta}\nabla f(\theta_{t}) 
        \Eb[z_{t+1} - z_{t}] & = \frac{-\alpha}{1 - \beta} \nabla f(\theta_t)
    \end{align*}
    For the last equation, since
    \begin{align*}
        z_{t+1}-z_t &= \frac{1}{1-\beta}(\theta_{t+1}-\theta_{t}) - \frac{\beta}{1-\beta}(\theta_{t}-\theta_{t-1}) \\ 
        &=
        % \frac{1}{1-\beta}(\theta_{t+1}-(\theta_{t}-\alpha m_{t+1})) - \frac{\beta}{1-\beta}(\theta_{t}-(\theta_{t-1} - \alpha m_t))
        -\frac{\alpha}{1-\beta}(m_{t+1}-\beta m_t)
    \end{align*}
    Take expectation and we have
    \begin{align*}
        \E{\norm{z_{t+1}-z_t}^2} &=
        % \E{\norm{\frac{1}{1-\beta}(\theta_{t+1}-(\theta_{t}-\alpha m_{t+1})) - \frac{\beta}{1-\beta}(\theta_{t}-(\theta_{t-1} - \alpha m_t)) - \frac{\alpha}{1-\beta}(m_{t+1}-\beta m_t)}^2} \\ &=
        % \frac{1}{(1-\beta)^2}\E{\norm{\theta_{t+1}-(\theta_{t}-\alpha m_{t+1})}^2} + \frac{\beta^2}{(1-\beta)^2}\E{\norm{\theta_{t}-(\theta_{t-1} - \alpha m_t)}^2} \\ &\quad + 
        \left(\frac{\alpha}{1-\beta}\right)^2\E{\norm{m_{t+1}-\beta m_t}^2} \\
        % &\quad - \frac{2\beta}{(1-\beta)^2}\E{<\theta_{t+1}-(\theta_{t}-\alpha m_{t+1}),\theta_{t}-(\theta_{t-1} - \alpha m_t)>} \\ &\quad -
        % \frac{2\alpha}{(1-\beta)^2}\E{<\theta_{t+1}-(\theta_{t}-\alpha m_{t+1}),m_{t+1}-\beta m_t>} \\ &\quad +
        % \frac{2\alpha\beta}{(1-\beta)^2}\E{<\theta_{t}-(\theta_{t-1} - \alpha m_t),m_{t+1}-\beta m_t>} \\ 
        &\le
        2\left(\frac{\alpha}{1-\beta}\right)^2 \left( \E{\norm{m_{t+1}-(\beta m_t + g_{t+1})}^2} + \E{\norm{g_{t+1}}^2}\right) \\
        % &~~~~ - 2\left(\frac{\alpha}{1-\beta}\right)^2 \E{\left\langle m_{t+1}-(\beta m_t + g_{t+1}),g_{t+1}\right\rangle} \\ 
        &\le
        2\left(\frac{\alpha}{1-\beta}\right)^2\left(\E{\norm{g_{t+1}}^2}  + \sigma_m^2\right).
    \end{align*}
\end{proof}

\begin{proof}[Proof of Theorem~\ref{thm:q-sgdm}]
    From Lemma 2, we have
    \begin{align*}
        \E{\norm{z_{t+1}-z_t}^2}\le
        2\left(\frac{\alpha}{1-\beta}\right)^2\left(\E{\norm{g_{t+1}}^2}  + \sigma_m^2\right).
    \end{align*}
    % And by Lemma 1, we know
    % \begin{align*}
    %     \E{\norm{g_{t+1}}^2}\le N\sigma_g^2 + N(N+2)\norm{\nabla{f}(\theta_{t})}^2 + N\sigma^2
    % \end{align*}
    Substituting Lemma 1 gives
    \begin{align}
        \label{eq:zdiff}
        \E{\norm{z_{t+1}-z_t}^2}
        \le 2\left(\frac{\alpha}{1-\beta}\right)^2\left(
        \norm{\nabla f(\theta_{t})}^2 + \sigma^2 + \sigma_m^2\right).
        % + \frac{1+2\beta^2}{(1-\beta)^2}\sigma_p^2
    \end{align}
    Suppose $\theta_*$ is the optimal parameter and $f_* = f(\theta_*)$ is the minimal objective value. First, we have
    \begin{align*}
    \norm{z_{t+1} - \theta_*}^2 & = \norm{z_{t} - \theta_*}^2 
    + 2 \left\langle z_t - \theta_*, z_{t+1} - z_t \right\rangle + \norm{z_{t+1} - z_t}^2
\end{align*}
Take expectation over the randomness in the $(t+1)-$th step, we have
\begin{align*}
    \Eb[\norm{z_{t+1} - \theta_*}^2] & = \norm{z_{t} - \theta_*}^2 
    - \frac{2\alpha}{1-\beta} \left\langle z_t - \theta_*, \nabla f(\theta_t) \right\rangle + \Eb[\norm{z_{t+1} - z_t}^2] \\
    & = \norm{z_{t} - \theta_*}^2 
    - \frac{2\alpha}{1-\beta} \left\langle \theta_t - \theta_*, \nabla f(\theta_t) \right\rangle \\
    & - \frac{2\alpha\beta}{(1-\beta)^2} \left\langle \theta_t - \theta_{t-1}, \nabla f(\theta_t)
    \right\rangle + \Eb[\norm{z_{t+1} - z_t}^2]
\end{align*}
    Since $f$ is continuously differentiable and L-smooth, we have the following inequalities. 
    \citep{2013Introductory}
    \begin{align}
        \left\langle \theta_t - \theta_*, \nabla f(\theta_t) \right\rangle \ge \frac{1}{L}\norm{\nabla f(\theta_t)}^2 \\
        \left\langle \theta_t - \theta_*, \nabla f(\theta_t) \right\rangle \ge f(\theta_t) - f_* + \frac{1}{2L}\norm{\nabla f(\theta_t)}^2 \\
        \left\langle \theta_t - \theta_{t-1}, \nabla f(\theta_t)\right\rangle \ge f(\theta_t) - f(\theta_{t-1})
    \end{align}
    Substitute them and get
\begin{align*}
    \Eb[\norm{z_{t+1} - \theta_*}^2] 
    & \le \norm{z_{t} - \theta_*}^2 
    - \frac{2\alpha (1 - \rho)}{L(1-\beta)} \norm{\nabla f(\theta_t)}^2 
    - \frac{2\alpha \rho}{1-\beta} (f(\theta_t) - f_*)\\
    & - \frac{\alpha \rho}{L(1-\beta)} \norm{\nabla f(\theta_t)}^2  - \frac{2\alpha \beta}{(1-\beta)^2} (f(\theta_t) - f(\theta_{t-1}))
    + \Eb[\norm{z_{t+1} - z_t}^2]
\end{align*}
    where $\rho\in(0,1]$ is a parameter used to balance the first two inequalities. 
    Denote $M = 2\left(\frac{\alpha}{1-\beta}\right)^2 \left( \sigma^2 + \sigma_m^2 \right)$. 
    Substitute Eq.~\ref{eq:zdiff} into this inequality and collect the terms, we get
\begin{align*}
    & \left( \frac{2\alpha \rho}{1-\beta} + \frac{2\alpha \beta}{(1-\beta)^2} \right) (f(\theta_t) - f_*) + \Eb[\norm{z_{t+1} - \theta_*}^2] \\
    \le &  \frac{2\alpha \beta}{(1-\beta)^2} \left( f(\theta_{t-1}) - f_*\right) 
    + \norm{z_t - \theta_*}^2 
    + \left( \frac{2\alpha^2}{(1 - \beta)^2}  - \frac{\alpha (2 - \rho)}{L(1-\beta)} \right) \norm{\nabla f(\theta_t)}^2 + M
\end{align*}
When $\alpha$ satisfies the condition $ \frac{2\alpha^2}{(1 - \beta)^2}  - \frac{\alpha (2 - \rho)}{L(1-\beta)} \le 0$, i.e. $ 0 \le \alpha \le \frac{(1 - \beta)(2 - \rho)}{2L}$, the term about $\norm{\nabla f(\theta_t)}^2$ is non-positive, thus we have
\begin{align*}
    & \left( \frac{2\alpha \rho}{1-\beta} + \frac{2\alpha \beta}{(1-\beta)^2} \right) (f(\theta_t) - f_*) + \Eb[\norm{z_{t+1} - \theta_*}^2] \\
    \le &  \frac{2\alpha \beta}{(1-\beta)^2} \left( f(\theta_{t-1}) - f_*\right) 
    + \norm{z_t - \theta_*}^2 + M
\end{align*}
Summing this inequality from 0 to $T - 1$ and taking full expectation gives
\begin{align*}
    & \frac{2\alpha \rho}{1-\beta} \sum_{i=0}^{T-1} \Eb[f(\theta_i) - f_*] 
    + \sum_{i=0}^{T-1} \left( \frac{2\alpha \beta}{(1-\beta)^2} \Eb[f(\theta_{i}) - f_*] + \Eb[\norm{z_{i+1} - \theta_*}^2]\right) \\
    \le & \sum_{i=0}^{T-1}  \left( \frac{2\alpha \beta}{(1-\beta)^2} \Eb[f(\theta_{i-1}) - f_*] + \Eb[\norm{z_{i} - \theta_*}^2]\right) + T\cdot M
\end{align*}
which implies that
\begin{align*}
    \frac{2\alpha \rho}{1-\beta} \sum_{i=0}^{T-1} \Eb[f(\theta_i) - f_*] 
    & \le \frac{2\alpha \beta}{(1-\beta)^2} (f(\theta_0) - f_*) + \norm{\theta_0 - \theta_*}^2 + T\cdot M
\end{align*}
Since $f$ is \emph{convex}, we have $T f(\Bar{{\theta}}_T) \le \frac{1}{T}\sum_{i=0}^{T-1} f(\theta_i))$.
Subsequently we have
\begin{align*}
    \Eb[f(\Bar{{\theta}}_T) - f_*] & \le \frac{1}{T}\left( \frac{\beta}{\rho(1-\beta)}(f(\theta_0) - f_*) + \frac{1-\beta}{2\alpha \rho}\norm{\theta_0 - \theta_*}^2 \right) \\
    & + \frac{1-\beta}{2\alpha \rho}M
\end{align*}
Finally, when $\alpha \in (0, \frac{1-\beta}{L}]$, we can take $\rho=1$, use L-smooth condition again and substitute $M$, which gives
\begin{align*}
    \Eb[f(\Bar{{\theta}}_T) - f_*] & \le \frac{1}{2T}\left( \frac{L\beta}{1-\beta} + \frac{1-\beta}{\alpha} \right) \norm{\theta_0 - \theta_*}^2\\
    & + \frac{\alpha \sigma^2}{(1-\beta)} 
    + \frac{\alpha\sigma_m^2}{(1-\beta)}
\end{align*}
% It's noted that when $N=1$, we get the basic quantized SGDM without gradient accumulation, whose convex convergence result is
% \begin{align*}
%     \Eb[f(\Bar{{\theta}}_T) - f_*] & \le \frac{1}{2T}\left( \frac{L\beta}{1-\beta} + \frac{1-\beta}{\alpha} \right) \norm{\theta_0 - \theta_*}^2\\
%     & + \frac{\alpha \sigma^2}{(1-\beta)} 
%     + \frac{\alpha\sigma_g^2}{(1-\beta)} 
%     + \frac{\alpha\sigma_m^2}{2(1-\beta)}
%     + \frac{(1+2\beta^2)\sigma_p^2}{2\alpha(1-\beta)}
% \end{align*}
\end{proof}
